# Supplementary material for: Energy Landscapes Enable Reliable Abstention in Retrieval-Augmented Large Language Models for Healthcare
Source: arXiv:2509.04482 ancillary file (2025-09-08)
Supplement: Supplementary file 1 [file supplementary_material.pdf]

# Energy Landscapes Enable Reliable Abstention in Retrieval-Augmented Large Language Models for Healthcare

Ravi Shankar<sup>1</sup>, Sheng Wong<sup>1</sup>, Lin Li<sup>2</sup>, Magdalena Bachmann<sup>3</sup>, Alex Silverthorne<sup>3</sup>, Beth Albert<sup>1</sup>, Gabriel Davis Jones<sup>1\*</sup>

<sup>1</sup>Oxford Digital Health Labs, Nuffield Department of Women’s and Reproductive Health, University of Oxford, Oxford, UK.

<sup>2</sup>OATML, Department of Computer Science, University of Oxford, Oxford, UK.

<sup>3</sup>Nuffield Department of Women’s and Reproductive Health, University of Oxford, Oxford, UK.

\*Corresponding author(s). E-mail(s): [gabriel.jones@wrh.ox.ac.uk](mailto:gabriel.jones@wrh.ox.ac.uk);

## 1 Supplementary

**Table 1:** Women’s health guidelines and publications used to prepare the questions corpus in this research.

| Title                                                                     | Synopsis                                                                                                                                                                                                             | Year | Authors                                                 | Publisher |
|---------------------------------------------------------------------------|----------------------------------------------------------------------------------------------------------------------------------------------------------------------------------------------------------------------|------|---------------------------------------------------------|-----------|
| Workplace-based assessment: a new approach to existing tools              | The article discusses the implementation challenges and revisions of workplace-based assessment (WPBA) tools in obstetrics and gynaecology, emphasizing the distinction between formative and summative assessments. | 2014 | William Parry-Smith, Ayesha Mahmud, Alex Landau, et al. | TOG       |
| Contraceptive methods and issues around the menopause: an evidence update | The publication discusses recent advances in contraceptive methods available to perimenopausal women, issues related to menopause, and the integration of hormone replacement therapy with contraception.            | 2017 | Shagaf H Bakour, Archana Hatti, Susan Whalen            | TOG       |
| Twin and triplet pregnancy                                                | This guideline covers care for pregnant women and pregnant people with a twin or triplet pregnancy, aiming to reduce complications and improve outcomes.                                                             | 2019 | –                                                       | NICE      |

Continued on next page

Table 1 – continued from previous page

| Title                                                                                       | Synopsis                                                                                                                                                                                                                                                                                                       | Year | Authors                                                                                                      | Publisher          |
|---------------------------------------------------------------------------------------------|----------------------------------------------------------------------------------------------------------------------------------------------------------------------------------------------------------------------------------------------------------------------------------------------------------------|------|--------------------------------------------------------------------------------------------------------------|--------------------|
| Management of sickle cell disease in pregnancy. A British Society for Haematology Guideline | This guideline describes the management of sickle cell disease in pregnancy, covering preconception, antenatal, intrapartum, and postnatal care, with updates on genetic diagnosis, medication review, and antenatal care recommendations.                                                                     | 2021 | Eugene Oteng-Ntim, Sue Pavord, Richard Howard, et al.                                                        | Br J Haematol      |
| Inducing labour                                                                             | This guideline covers the circumstances for inducing labour, methods of induction, assessment, monitoring, pain relief, and managing complications to improve advice and care for pregnant women considering or undergoing induction of labour.                                                                | 2021 | –                                                                                                            | NICE               |
| Saving Lives, Improving Mothers' Care State of the Nation Report                            | The report presents surveillance findings and lessons learned to inform maternity care from the UK and Ireland Confidential Enquiries into Maternal Deaths, focusing on thrombosis, thromboembolism, malignancy, ectopic pregnancy, and the care of recent migrants with language difficulties from 2020-2022. | 2024 | MBRRACE-UK                                                                                                   | NPEU, Univ. Oxford |
| Laparoscopy in urogynaecology                                                               | This article discusses the advancements and challenges in laparoscopic urogynaecological surgery, focusing on procedures for prolapse and stress incontinence, and highlights the importance of training and patient choice.                                                                                   | 2018 | Rajvinder Khasriya, Arvind Vashisht, Alfred Cutner                                                           | TOG                |
| Failed hysteroscopy and further management strategies                                       | This article explores various methods to overcome cervical stenosis in hysteroscopy, highlighting techniques such as pharmacological, mechanical, hygroscopic, and ultrasound-guided dilatation.                                                                                                               | 2016 | Sophie Relph, Tessa Lawton, Mark Broadbent, et al.                                                           | TOG                |
| An overview of assisted reproductive technology procedures                                  | This article provides a comprehensive overview of assisted reproductive technology (ART) procedures, discussing key steps, individualised treatment protocols, and multidisciplinary management for fertility issues.                                                                                          | 2018 | Harish M Bhandari, Meenakshi K Choudhary, Jane A Stewart                                                     | TOG                |
| Multiple Pregnancies Following Assisted Conception                                          | This paper discusses the high rates of multiple pregnancies following IVF and the measures taken to reduce these rates, highlighting the importance of elective single embryo transfer (eSET) and the progress made in the UK.                                                                                 | 2018 | T El-Toukhy, S Bhattacharya, VA Akande                                                                       | RCOG               |
| Making Abortion Safe                                                                        | The publication outlines best practices in abortion care to ensure safe and effective services, emphasizing evidence-based clinical practice and addressing barriers to safe abortion globally.                                                                                                                | 2022 | Updated by Sharon Cameron, Jayne Kavanagh, Patricia A Lohr; originally developed by Anna Glasier and others. | RCOG               |
| Evaluating misoprostol and mechanical methods for induction of labour                       | This paper reviews the use of misoprostol and mechanical methods for induction of labour, comparing their safety and efficacy to the standard drug, dinoprostone.                                                                                                                                              | 2022 | Andrew D. Weeks, Kate Lightly, Ben W. Mol, et al.                                                            | RCOG               |
| Does ovarian cystectomy pose a risk to ovarian reserve and fertility?                       | This article reviews the impact of ovarian cystectomy on ovarian reserve and fertility, discussing factors such as cyst type, size, and surgical techniques that influence outcomes.                                                                                                                           | 2020 | Neerujah Balachandren, Ephiah Yasmin, Dimitrios Mavrelou, et al.                                             | TOG                |
| Thromboembolic Disease in Pregnancy and the Puerperium: Acute Management                    | This guideline provides information on the immediate investigation and management of venous thromboembolism (VTE) in pregnant women and those in the puerperium, emphasizing the use of low-molecular-weight heparin (LMWH) and the importance of objective testing.                                           | 2015 | –                                                                                                            | RCOG               |
| Caesarean section at full dilatation: incidence, impact and current management              | This article reviews the increasing incidence of caesarean sections performed at full dilatation, associated maternal and neonatal risks, and current management practices.                                                                                                                                    | 2014 | Nicola Vousden, Zillah Cargill, Annette Briley, et al.                                                       | TOG                |

Continued on next page

Table 1 – continued from previous page

| Title                                                                                              | Synopsis                                                                                                                                                                                                                                                              | Year | Authors                                                           | Publisher                                           |
|----------------------------------------------------------------------------------------------------|-----------------------------------------------------------------------------------------------------------------------------------------------------------------------------------------------------------------------------------------------------------------------|------|-------------------------------------------------------------------|-----------------------------------------------------|
| Androgens in postmenopausal women                                                                  | The article explores the role of androgen therapy in improving sexual wellbeing and libido in postmenopausal women, discussing the physiology of testosterone, its effects, and the potential benefits and risks of therapy.                                          | 2022 | Kugajeevan Vigneswaran, Haitham Hamoda                            | TOG                                                 |
| Operative laparoscopy in advanced pregnancy beyond 20 weeks                                        | The article explores the benefits and technical challenges of performing laparoscopic procedures in advanced pregnancy, emphasizing its feasibility and safety even beyond 20 weeks of gestation.                                                                     | 2020 | Suzanna Morton, Nina Cooper, Jasmin Walravens-Evans, et al.       | TOG                                                 |
| Spontaneous preterm birth prevention in multiple pregnancy                                         | The article reviews the burden of preterm birth in multiple pregnancies and evaluates the effectiveness of various interventions, such as cervical cerclage, progesterone, and cervical pessary, in preventing preterm birth in twin pregnancies.                     | 2018 | Sarah R Murray, Sarah J Stock, Shona Cowan, et al.                | TOG                                                 |
| Endometriosis and irritable bowel syndrome: a dilemma for the gynaecologist and gastroenterologist | This article explores the overlap between endometriosis and irritable bowel syndrome, highlighting the challenges in diagnosis and management due to their similar symptomatology and the importance of collaboration between gastroenterologists and gynaecologists. | 2016 | Basma Issa, Laura Ormesher, Peter J Whorwell, et al.              | TOG                                                 |
| Recent trends in molecular testing and maintenance targeted therapies in ovarian cancer            | This review discusses the advancements in molecular testing and maintenance therapies, particularly PARP inhibitors, for high-grade serous ovarian cancer, highlighting the role of homologous recombination deficiency in treatment outcomes.                        | 2023 | Ahmed Darwish, Osnat Elyashiv, Radha Graham, et al.               | TOG                                                 |
| Diagnosis, pathophysiology and management of premenstrual syndrome                                 | This article provides an overview of premenstrual syndrome (PMS), including its diagnosis, pathophysiology, and management strategies, in line with the RCOG Green-top Guideline.                                                                                     | 2015 | Sally Walsh, Elgerta Ismaili, Bushra Naheed, et al.               | TOG                                                 |
| Tuberculosis in pregnancy                                                                          | This article discusses the impact of tuberculosis on pregnancy, including its diagnosis, management, and the challenges posed by co-infections and drug resistance.                                                                                                   | 2023 | Ainharan Raveendran, Anish Keepanasseril, Ravi Kumar Balu, et al. | TOG                                                 |
| Thromboprophylaxis in gynaecology: a review of current evidence                                    | This article reviews the current evidence on thromboprophylaxis in gynaecology, highlighting the risks, recommendations, and gaps in guidance for preventing venous thromboembolism in gynaecological practice.                                                       | 2023 | Divya Nambiar, Jecko Thachil, Wai Yoong, et al.                   | TOG                                                 |
| 2021 FIGO Staging System for Vulvar Cancer: Summary and comparison with 2009 FIGO Staging System   | The article discusses the revisions in the 2021 FIGO staging system for vulvar cancer, comparing it with the 2009 system and highlighting key changes in staging criteria.                                                                                            | 2021 | Brian Rous, Raji Ganesan, Asma Faruqi, et al.                     | International Journal of Gynaecology and Obstetrics |
| Maternal sepsis update: current management and controversies                                       | This article discusses the current management, controversies, and recent updates in the management of maternal sepsis, highlighting the complexities of diagnosis and the importance of translational research and clinical trials.                                   | 2020 | Orene Greer, Nishel Mohan Shah, Mark R Johnson                    | TOG                                                 |
| Outpatient Hysteroscopy                                                                            | This guideline provides evidence-based information on outpatient hysteroscopy, focusing on minimizing pain and optimizing patient experience, with updates on operative procedures, infection prevention, and training.                                               | 2024 | Prathiba M. De Silva, Paul P. Smith, Natalie A. M. Cooper, et al. | RCOG                                                |
| Complications of caesarean section                                                                 | The article reviews the incidence, presentation, and management of complications associated with caesarean sections, including haemorrhage, sepsis, and visceral injuries.                                                                                            | 2016 | Alexander Field, Rahim Haloob                                     | TOG                                                 |
| Best Practice in Outpatient Hysteroscopy                                                           | This guideline provides clinicians with evidence-based information on outpatient hysteroscopy, focusing on minimizing pain and optimizing the woman's experience.                                                                                                     | 2011 | –                                                                 | RCOG                                                |

Continued on next page

Table 1 – continued from previous page

| Title                                                                                            | Synopsis                                                                                                                                                                                                                                                             | Year | Authors                                                       | Publisher                                 |
|--------------------------------------------------------------------------------------------------|----------------------------------------------------------------------------------------------------------------------------------------------------------------------------------------------------------------------------------------------------------------------|------|---------------------------------------------------------------|-------------------------------------------|
| Understanding the Mental Capacity Act 2005: a guide for clinicians                               | This article provides an overview of the Mental Capacity Act 2005, explaining its implications for clinicians in assessing mental capacity, making advance decisions, and understanding the role of Lasting Powers of Attorney.                                      | 2010 | Nick Nicholas, Sotiris Nicholas                               | TOG                                       |
| Congenital Cytomegalovirus Infection: Update on Treatment                                        | This paper provides an update on the treatment of congenital cytomegalovirus infection, summarizing issues around screening, diagnosis, and treatment during pregnancy.                                                                                              | 2017 | Khalil A, Heath P, Jones C, et al.                            | RCOG                                      |
| Surgical site infections: prevention and treatment                                               | This guideline covers preventing and treating surgical site infections in adults, young people, and children undergoing surgical procedures involving a cut through the skin, focusing on methods used before, during, and after surgery to minimize infection risk. | 2019 | –                                                             | NICE                                      |
| Hypertension in pregnancy: diagnosis and management                                              | This guideline covers diagnosing and managing hypertension, including pre-eclampsia, during pregnancy, labour, and birth, aiming to improve care for women and their babies.                                                                                         | 2019 | –                                                             | NICE                                      |
| Menopause and mental health                                                                      | The article explores the prevalence and management of mental health issues during menopause, emphasizing the role of lifestyle changes, hormone replacement therapy, and cognitive behavioral therapy.                                                               | 2023 | Ajay Swaminathan, Peter Lepping, Geeta Kumar                  | TOG                                       |
| Best practice in post-abortion contraception                                                     | The publication provides guidelines on starting contraception methods at the time of an abortion, emphasizing the importance of person-centered care and shared decision-making in post-abortion contraceptive counseling.                                           | 2022 | Jayne Kavanagh, Sharon Cameron, Roua Abu Hurayra, et al.      | RCOG                                      |
| 2023 UK National Guideline on the Management of Vulval Conditions                                | This guideline provides recommendations for managing various vulval disorders, focusing on conditions that may present to Genitourinary Medicine clinics and offering guidance for diagnostic tests and treatment regimens.                                          | 2023 | Sarah K Edwards, Fiona Lewis, Imali Fernando, et al.          | British Association Sexual Health and HIV |
| Adrenal disease and pregnancy: an overview                                                       | This article provides an overview of adrenal diseases complicating pregnancy, discussing their clinical features, diagnosis, and management to optimize maternal and fetal outcomes.                                                                                 | 2021 | Mayada Ahmed, Mohammed Bashir, Gbemisola O Okunoye, et al.    | TOG                                       |
| Surgical causes of acute abdominal pain in pregnancy                                             | This article discusses the differential diagnoses and management of surgical causes of acute abdominal pain in pregnant women, emphasizing the need for a structured assessment and collaborative multispecialty practice.                                           | 2019 | Natalie Woodhead, Oga Nkwam, Virginia Caddick, et al.         | TOG                                       |
| Management of Female Malignant Ovarian Germ Cell Tumours                                         | This paper discusses the management of female malignant ovarian germ cell tumours, highlighting the importance of early diagnosis, multi-agent chemotherapy, and a multidisciplinary approach to improve outcomes.                                                   | 2016 | Professor JA Tidy, Professor RE Coleman, Dr RA Harvey, et al. | RCOG                                      |
| Fertility on ice: an overview of fertility preservation for children and adolescents with cancer | The article reviews current options for fertility preservation for children and adolescents with cancer, discussing methods such as oocyte cryopreservation, ovarian tissue cryopreservation, sperm cryopreservation, and testicular tissue cryopreservation.        | 2021 | Lucia Hartigan, Louise E Glover, Mary Wingfield               | TOG                                       |
| PRESENTING INFORMATION ON RISK                                                                   | This clinical governance advice provides guidance on effectively communicating risk to patients, emphasizing the importance of perception, decision-making, and personalized communication.                                                                          | –    | Dr A David MRCOG, London                                      | RCOG                                      |
| Outflow tract disorders of the female genital tract                                              | The article discusses congenital anomalies of the female genital tract, emphasizing the importance of embryological knowledge for diagnosis and management, and highlights the need for specialist care in complex cases like MRKH syndrome.                         | 2013 | D Keith Edmonds, Gillian L Rose                               | TOG                                       |

Continued on next page

Table 1 – continued from previous page

| Title                                                                                                                | Synopsis                                                                                                                                                                                                                                                   | Year | Authors                                                                                                            | Publisher                                                                                                     |
|----------------------------------------------------------------------------------------------------------------------|------------------------------------------------------------------------------------------------------------------------------------------------------------------------------------------------------------------------------------------------------------|------|--------------------------------------------------------------------------------------------------------------------|---------------------------------------------------------------------------------------------------------------|
| Induction of Labour at Term in Older Mothers                                                                         | This paper discusses the risks and benefits of inducing labour at term in older mothers, considering factors such as stillbirth risk, neonatal mortality, and the potential for increased surgical interventions.                                          | 2013 | Ms MK Dhanjal FRCOG, Ms A Kenyon MRCOG                                                                             | RCOG                                                                                                          |
| Operative Vaginal Delivery                                                                                           | This paper provides advice for clinicians on obtaining consent for women undergoing operative vaginal delivery, ensuring they receive consistent and adequate information for consent.                                                                     | 2010 | Dr LC Edozien FRCOG with the support of the Consent Group of the Royal College of Obstetricians and Gynaecologists | RCOG                                                                                                          |
| Preterm labour and birth                                                                                             | This guideline covers the care of women with a singleton pregnancy at increased risk of, or with symptoms and signs of, preterm labour, aiming to reduce risks for the baby and describing treatments to prevent or delay early labour and birth.          | 2022 | –                                                                                                                  | NICE                                                                                                          |
| Identification and management of fetal anaemia: a practical guide                                                    | This article provides an overview of the identification and management of fetal anaemia, focusing on screening, diagnosis, and treatment strategies to improve outcomes in affected pregnancies.                                                           | 2021 | James Castleman, Leo Gurney, Mark Kilby, et al.                                                                    | TOG                                                                                                           |
| Preventing Entry-Related Gynaecological Laparoscopic Injuries                                                        | This guideline aims to highlight strategies to reduce complications during laparoscopic surgery, particularly during the blind insertion of needles, trocars, and cannulae.                                                                                | –    | Professor CJG Sutton FRCOG, Mr K Philips FRCOG, Dr DE Parkin FRCOG, et al.                                         | RCOG                                                                                                          |
| Menopause: identification and management                                                                             | This guideline covers identifying and managing menopause, including in people with premature ovarian insufficiency, aiming to improve the consistency of support and information provided to people experiencing menopause.                                | 2024 | –                                                                                                                  | NICE                                                                                                          |
| The diagnosis and treatment of malaria in pregnancy                                                                  | This guideline provides clinicians with up-to-date, evidence-based information on the diagnosis and treatment of malaria in pregnancy, particularly in the UK context.                                                                                     | 2010 | –                                                                                                                  | RCOG                                                                                                          |
| BSGE/ESGE guideline on management of fluid distension media in operative hysteroscopy                                | This article provides guidelines on the management of fluid distension media in operative hysteroscopy, highlighting risks, prevention, and management of complications from excessive fluid absorption.                                                   | 2018 | Sameer Umranikar, Ertan Saridogan, T Justin Clark, et al.                                                          | TOG                                                                                                           |
| Recurrent urinary tract infections: a critical review of the currently available treatment options                   | This article reviews the current treatment options for recurrent urinary tract infections (rUTIs), highlighting the clinical and socio-economic burden, antibiotic resistance issues, and the need for more research into effective management strategies. | 2020 | Mike Negus, Christian Phillips, Richard Hindley                                                                    | TOG                                                                                                           |
| MBRRACE-UK Perinatal Mortality Surveillance: UK Perinatal Deaths of Babies Born in 2022 - State of the Nation Report | This report provides an analysis of perinatal mortality rates in the UK for babies born in 2022, highlighting trends, causes of death, and variations by gestational age, socioeconomic status, and ethnicity.                                             | 2024 | Gallimore ID, Matthews RJ, Page GL, et al.                                                                         | The Infant Mortality and Morbidity Studies, Department of Population Health Sciences, University of Leicester |
| Management of ovarian cysts in children and adolescents                                                              | This review provides an evidence-based tool for the management of ovarian cysts in children and adolescent girls, highlighting common presentations, diagnosis, management options, and follow-up.                                                         | 2020 | Neelam Potdar, Rekha N Pillai, Christina A Oppenheimer                                                             | TOG                                                                                                           |

Continued on next page

Table 1 – continued from previous page

| Title                                                                                                            | Synopsis                                                                                                                                                                                                                                                       | Year | Authors                                                          | Publisher |
|------------------------------------------------------------------------------------------------------------------|----------------------------------------------------------------------------------------------------------------------------------------------------------------------------------------------------------------------------------------------------------------|------|------------------------------------------------------------------|-----------|
| Preconception health in the well woman                                                                           | The article discusses the importance of preconception care in improving maternal and neonatal outcomes, highlighting the impact of socioeconomic factors, nutrition, and lifestyle on reproductive health.                                                     | 2022 | Charlotte Brooks, Prasanna Supramaniam, Raj Monica Mittal        | TOG       |
| Ectopic pregnancy and miscarriage: diagnosis and initial management                                              | This guideline covers diagnosing and managing ectopic pregnancy and miscarriage in women with complications in early pregnancy, aiming to improve diagnosis and support to limit psychological impact.                                                         | 2019 | –                                                                | NICE      |
| Cell-free fetal DNA-based noninvasive prenatal testing of aneuploidy                                             | This article reviews the use of cell-free fetal DNA-based noninvasive prenatal testing (NIPT) for aneuploidy, discussing its accuracy, limitations, ethical issues, and potential role in antenatal care.                                                      | 2017 | Fiona L Mackie, Stephanie Allen, R Katie Morris, et al.          | TOG       |
| Epilepsy in Pregnancy                                                                                            | This guideline provides recommendations on the care of women with epilepsy during the prepregnancy, antepartum, intrapartum, and postpartum periods, focusing on maternal and fetal outcomes.                                                                  | 2016 | –                                                                | RCOG      |
| Caesarean birth                                                                                                  | This guideline covers when to offer and discuss caesarean birth, procedural aspects of the operation, and care after caesarean birth to improve the consistency and quality of care for women and pregnant people considering or having had a caesarean birth. | 2021 | –                                                                | NICE      |
| Subclinical hypothyroidism and antithyroid autoantibodies in women with subfertility or recurrent pregnancy loss | This Scientific Impact Paper discusses thyroid testing and management of mild thyroid problems and thyroid antibodies in women with subfertility or recurrent miscarriages, suggesting potential treatment with thyroxine tablets.                             | 2022 | Rima K. Dhillon-Smith, Kristien Boelaert, Yadava B. Jeve, et al. | RCOG      |
| Hormone replacement therapy following treatment of gynaecological malignancies                                   | The article reviews the safety and management of hormone replacement therapy (HRT) in women who have undergone treatment for various gynaecological malignancies, emphasizing the need for an evidence-based approach to managing menopausal symptoms.         | 2019 | Alison Richardson, Julie Ayres, Mike Cust, et al.                | TOG       |
| Fowler's syndrome: a primary disorder of urethral sphincter relaxation                                           | The article discusses Fowler's syndrome, a condition characterized by urinary retention in young women due to urethral sphincter dysfunction, and explores diagnostic and treatment options such as sacral neuromodulation and botulinum toxin injections.     | 2018 | Jalesh N Panicker, Mahreen Pakzad, Clare J Fowler                | TOG       |
| Endometrial pathology in the postmenopausal woman – an evidence based approach to management                     | This article provides an overview of the identification, investigation, and management of endometrial pathology in postmenopausal women, focusing on both symptomatic and asymptomatic cases.                                                                  | 2015 | Mohamed Otify, Joanna Fuller, Jackie Ross, et al.                | TOG       |
| Perioperative care in adults                                                                                     | This guideline covers care for adults having elective or emergency surgery, including dental surgery, and includes recommendations on preparing for surgery, keeping people safe during surgery, and pain relief during recovery.                              | 2020 | –                                                                | NICE      |
| Urinary incontinence and pelvic organ prolapse in women: management                                              | This guideline covers assessing and managing urinary incontinence and pelvic organ prolapse in women aged 18 and over, including complications associated with mesh surgery for these conditions.                                                              | 2019 | –                                                                | NICE      |
| Present status and advances in bladder pain syndrome: central sensitisation and the urinary microbiome           | The article explores the pathophysiology of bladder pain syndrome, focusing on central sensitisation and the role of the urinary microbiome, and discusses potential treatment strategies.                                                                     | 2022 | Ifeoma Offiah, Rosie Campbell, Anupreet Dua, et al.              | TOG       |

Continued on next page

Table 1 – continued from previous page

| Title                                                                                             | Synopsis                                                                                                                                                                                                                            | Year | Authors                                                                | Publisher                           |
|---------------------------------------------------------------------------------------------------|-------------------------------------------------------------------------------------------------------------------------------------------------------------------------------------------------------------------------------------|------|------------------------------------------------------------------------|-------------------------------------|
| Fibroids in pregnancy: management and outcomes                                                    | This article discusses the complications and management options for fibroids during pregnancy, including surgical interventions and their impact on pregnancy outcomes.                                                             | 2018 | Karan Sampat, Djavid I Alleemudder                                     | TOG                                 |
| Management of gynaecological cancer in pregnancy                                                  | This article summarises the management and outcomes of gynaecological cancers in relation to pregnancy, discussing pre-existing cancer, diagnosis, and postpartum management.                                                       | 2017 | Susnata China, Yashashwi Sinha, Deepali Sinha, et al.                  | TOG                                 |
| Laser treatment for genitourinary syndrome of menopause                                           | This paper reviews the evidence for laser therapy as a treatment for genitourinary syndrome of menopause, highlighting its potential benefits and the need for further research before widespread adoption.                         | 2022 | Christian Phillips, Timothy Hillard, Stefano Salvatore, et al.         | RCOG                                |
| 2014 UK national guideline on the management of vulval conditions                                 | This guideline provides recommendations for the management of various vulval disorders, focusing on non-infective conditions and offering guidance for genitourinary medicine clinics.                                              | 2014 | Sarah K Edwards, Christine M Bates, Fiona Lewis, et al.                | International Journal of STD & AIDS |
| Cervical cancer in pregnancy: diagnosis, staging and treatment                                    | This article discusses the diagnosis, staging, and treatment of cervical cancer during pregnancy, emphasizing the complexity and necessity of a multidisciplinary approach.                                                         | 2022 | Tamara Howe, Kate Lankester, Tony Kelly, et al.                        | TOG                                 |
| Chemical Exposures During Pregnancy: Dealing with Potential, but Unproven, Risks to Child Health  | This paper raises awareness about the potential risks of chemical exposures during pregnancy and breastfeeding, aiming to equip women with sufficient information to make informed decisions regarding chemical exposure.           | 2013 | Dr M Bellingham PhD, Glasgow and Professor RM Sharpe, PhD FRSE, et al. | RCOG                                |
| Diagnosis and management of liver masses in pregnancy                                             | This article reviews the diagnosis and management of liver masses in pregnancy, emphasizing the importance of multidisciplinary collaboration and the challenges posed by hormonal influences and imaging techniques.               | 2016 | James Milburn, Mairead Black, Irfan Ahmed, et al.                      | TOG                                 |
| Optimum Surgery in Advanced-stage Ovarian Cancer                                                  | The paper discusses the role and timing of surgery in advanced-stage ovarian cancer, highlighting the need for further trials to determine the optimal surgical approach.                                                           | 2011 | Mr R Naik FRCOG, Mr GAJ McIndoe MRCOG, Mr TAJ Mould FRCOG, et al.      | RCOG                                |
| Preventing adhesions in laparoscopic surgery: the role of anti-adhesion agents                    | This article reviews the pathophysiology of adhesion formation after laparoscopic surgery and evaluates the effectiveness and cost implications of various anti-adhesion agents.                                                    | 2019 | Mehrnoosh Aref-Adib, Timothy Phan, Alexandre Ades                      | TOG                                 |
| Guidance 7. Job roles: lead clinician colposcopist and lead colposcopy nurse                      | This guidance outlines the roles and responsibilities of the lead clinician colposcopist and lead colposcopy nurse in ensuring the quality and effectiveness of colposcopy services.                                                | 2024 | –                                                                      | NHS England                         |
| The clinical applications of interventional radiological techniques in obstetrics and gynaecology | This article reviews the use of interventional radiology techniques in obstetrics and gynaecology, highlighting their applications, benefits, and risks compared to traditional surgical methods.                                   | 2023 | Rhianna Davies, Michael Parker, Avi Basu, et al.                       | TOG                                 |
| Non-invasive Prenatal Testing for Chromosomal Abnormality using Maternal Plasma DNA               | This paper reviews the issues and implications of non-invasive prenatal testing (NIPT) using maternal plasma DNA for detecting chromosomal abnormalities, offering a safer alternative to invasive procedures.                      | 2014 | Professor PW Soothill, Professor YMD Lo                                | RCOG                                |
| Review of advanced energy devices for the minimal access gynaecologist                            | This article reviews advanced energy devices used in minimal access gynaecology, discussing their biophysics, advantages, disadvantages, and safety considerations to aid gynaecologists in selecting optimal surgical instruments. | 2021 | Gemma L Bentham, Jessica Preshaw                                       | TOG                                 |

Continued on next page

Table 1 – continued from previous page

| Title                                                                                                                 | Synopsis                                                                                                                                                                                                                                                     | Year | Authors                                                                                                                      | Publisher |
|-----------------------------------------------------------------------------------------------------------------------|--------------------------------------------------------------------------------------------------------------------------------------------------------------------------------------------------------------------------------------------------------------|------|------------------------------------------------------------------------------------------------------------------------------|-----------|
| Management of delivery when malposition of the fetal head complicates the second stage of labour                      | The article discusses the management of fetal head malposition during the second stage of labour, highlighting the need for advanced training and guidelines for rotational vaginal deliveries to reduce caesarean section rates and associated morbidities. | 2015 | Nicola Tempest, Kate Navaratnam, Dharani K Hapangama                                                                         | TOG       |
| Intrauterine contraception                                                                                            | The article discusses the types, benefits, and challenges of intrauterine contraception, emphasizing the need for comprehensive knowledge to dispel myths and provide effective counselling.                                                                 | 2021 | Joanne Ritchie, Nicholas Phelan, Paula Briggs                                                                                | TOG       |
| Obtaining Valid Consent                                                                                               | This guidance provides a framework for obtaining valid consent in obstetrics and gynaecology, emphasizing informed decision-making and patient autonomy.                                                                                                     | 2015 | Mr EP Morris FRCOG, Norwich                                                                                                  | RCOG      |
| Venous thromboembolism in over 16s: reducing the risk of hospital-acquired deep vein thrombosis or pulmonary embolism | This guideline covers assessing and reducing the risk of venous thromboembolism (VTE) in people aged 16 and over in hospital, aiming to help healthcare professionals identify those most at risk and describe interventions to reduce VTE risk.             | 2018 | –                                                                                                                            | NICE      |
| Long-acting reversible contraception                                                                                  | This guideline covers long-acting reversible contraception and aims to increase its use by improving the information given to women about their contraceptive choices.                                                                                       | 2019 | –                                                                                                                            | NICE      |
| Autopsy in the event of maternal death – a UK perspective                                                             | The article discusses the role of autopsies in understanding maternal deaths in the UK, highlighting legal requirements, clinical pathologies, and the importance of accurate autopsy data in reducing maternal mortality.                                   | 2019 | Sebastian Lucas                                                                                                              | TOG       |
| Sentinel lymph node mapping in the modern management of gynaecological malignancy                                     | This article reviews the role of sentinel lymph node mapping as an alternative to systematic lymphadenectomy in the surgical staging of gynaecological malignancies, focusing on its application in vulval, cervical, and endometrial cancers.               | 2023 | Anna Collins, Andrew Phillips                                                                                                | TOG       |
| Consent Advice No. 1: Diagnostic Hysteroscopy Under General Anaesthesia                                               | This guidance provides advice for clinicians on obtaining consent from women undergoing diagnostic hysteroscopy under general anaesthesia, ensuring they receive consistent and adequate information.                                                        | 2008 | Dr MD Read FRCOG, Gloucester, with the support of the Consent Group of the Royal College of Obstetricians and Gynaecologists | RCOG      |
| Sexual assault                                                                                                        | This article highlights the prevalence and impact of sexual assault on women's health, discussing immediate care, forensic examination, and long-term needs for victims.                                                                                     | 2018 | Lisa Long, Bernadette Butler                                                                                                 | TOG       |
| Peripartum cardiomyopathy                                                                                             | The article discusses the increasing incidence, pathogenesis, clinical presentation, and management of peripartum cardiomyopathy, emphasizing the importance of early diagnosis and multidisciplinary care.                                                  | 2021 | Akshatha Kulkarni, Gareth Squire, Kai Hogrefe, et al.                                                                        | TOG       |
| Management of adnexal masses in pregnancy                                                                             | The article discusses the prevalence, classification, assessment, and management of adnexal masses in pregnancy, highlighting the importance of differentiating between benign and malignant lesions and the role of multidisciplinary approaches.           | 2017 | Aderemi O Alalade, Hemant Maraj                                                                                              | TOG       |
| Female genital mutilation in the UK: what are the barriers to prosecution?                                            | This article discusses the barriers to prosecuting female genital mutilation (FGM) in the UK, the efficacy of legislative changes, and suggests future actions to improve prosecution rates.                                                                 | –    | Jessica Gubbin, Erna Bayar, I G Finlay (Baroness Finlay of Llandaff)                                                         | –         |

Continued on next page

**Table 1 – continued from previous page**

| Title                                                                                                                      | Synopsis                                                                                                                                                                                                                                                                     | Year | Authors                                                                                                                                 | Publisher |
|----------------------------------------------------------------------------------------------------------------------------|------------------------------------------------------------------------------------------------------------------------------------------------------------------------------------------------------------------------------------------------------------------------------|------|-----------------------------------------------------------------------------------------------------------------------------------------|-----------|
| Fetal surgery for open spina bifida                                                                                        | The article discusses the benefits and risks of open fetal surgery for spina bifida, highlighting improved outcomes for the child despite increased risks of prematurity and maternal morbidity.                                                                             | 2019 | Adalina Sacco, Fred Ushakov, Dominic Thompson, et al.                                                                                   | TOG       |
| Vaginal Surgery for Prolapse                                                                                               | This guidance provides advice for clinicians on obtaining consent from women undergoing vaginal surgery for prolapse, ensuring consistent and adequate information is given for informed consent.                                                                            | 2009 | Mr ADG Roberts FRCOG, Burton upon Trent, with the support of the Consent Group of the Royal College of Obstetricians and Gynaecologists | RCOG      |
| Evidence to Support the Clinical Utility of Prenatal Exome Sequencing in Evaluation of the Fetus with Congenital Anomalies | This paper reviews the evidence supporting the use of prenatal exome sequencing for diagnosing genetic causes of congenital anomalies in fetuses, highlighting its potential to improve diagnostic rates and inform clinical practice.                                       | 2021 | F Mone, DJ McMullan, D Williams, et al.                                                                                                 | RCOG      |
| Uterine rupture: a revisit                                                                                                 | The article reviews the causes, risk factors, and management of uterine rupture, emphasizing the need for increased awareness and proper risk assessment to prevent this serious complication.                                                                               | 2010 | Madhavi Manoharan, Rekha Wuntakal, Katrina Erskine                                                                                      | TOG       |
| Pre-implantation genetic testing for aneuploidy: the past, present and future                                              | This article reviews the evolution, current practices, and future implications of pre-implantation genetic testing for aneuploidy (PGT-A) in assisted reproduction, highlighting technological advancements and clinical outcomes.                                           | 2020 | Ariadne L'Heveder, Benjamin P Jones, Roy Naja, et al.                                                                                   | TOG       |
| Management of Inherited Bleeding Disorders in Pregnancy                                                                    | This guideline provides comprehensive management strategies for pregnant women with inherited bleeding disorders, focusing on haemophilia, von Willebrand disease, and other rare bleeding disorders, emphasizing multidisciplinary care and individualized treatment plans. | 2017 | Pavord S, Rayment R, Madan B, et al.                                                                                                    | RCOG      |
| Guidelines for the Diagnosis and Management of Vulval Carcinoma                                                            | This document provides updated guidelines for the diagnosis and management of vulval carcinoma, emphasizing surgical treatment, the role of radiotherapy and chemotherapy, and the importance of multidisciplinary care.                                                     | 2014 | Professor DM Luesley, Miss A Tristram, Dr R Ganesan, et al.                                                                             | RCOG      |
| Extra corporeal membrane oxygenation (ECMO) in pregnant and postpartum women                                               | This article reviews the use of extracorporeal membrane oxygenation (ECMO) in pregnant and postpartum women, highlighting its application in cases of severe cardiac or respiratory failure and the complexities involved in managing such cases.                            | 2023 | Anna Richmond, Farah Siddiqui, Caroline Sampson, et al.                                                                                 | TOG       |
| Excision of endometriosis – optimising surgical techniques                                                                 | This article reviews principles and techniques for the optimal and safe excision of endometriosis, emphasizing a structured approach using the SOSURE framework.                                                                                                             | 2021 | Kyle Fleischer, Ahmed El Gohari, Matthew Erritty, et al.                                                                                | TOG       |
| Labour Ward Solutions                                                                                                      | This document provides guidance for implementing RCOG and CNST maternity standards, focusing on expanding consultant presence on the labour ward and addressing related challenges.                                                                                          | 2009 | Mr Edward Morris FRCOG, Dr Tahir Mahmood FRCOG, Mrs Charnjit Dhillon                                                                    | RCOG      |
| Labour Ward Solutions                                                                                                      | This document provides guidance on expanding consultant presence on labour wards, addressing challenges and offering practical solutions for implementing RCOG and CNST maternity standards.                                                                                 | 2009 | Mr Edward Morris FRCOG, Dr Tahir Mahmood FRCOG, Mrs Charnjit Dhillon                                                                    | RCOG      |

Continued on next page

Table 1 – continued from previous page

| Title                                                                                                                  | Synopsis                                                                                                                                                                                                                                                                       | Year | Authors                                                        | Publisher |
|------------------------------------------------------------------------------------------------------------------------|--------------------------------------------------------------------------------------------------------------------------------------------------------------------------------------------------------------------------------------------------------------------------------|------|----------------------------------------------------------------|-----------|
| Complications of assisted reproductive treatment and the factors influencing reproductive outcome                      | This article reviews the complications associated with assisted reproductive technology (ART) treatment and examines factors influencing reproductive outcomes, including risks such as ovarian hyperstimulation syndrome, multiple pregnancies, and potential cancer risks.   | 2018 | Harish M Bhandari, Meenakshi K Choudhary, Jane A Stewart       | TOG       |
| Investigation and Care of a Small-for-Gestational-Age Fetus and a Growth Restricted Fetus (Green-top Guideline No. 31) | This guideline provides evidence-based advice for clinicians on the investigation and management of small-for-gestational-age (SGA) and growth-restricted fetuses, including risk factors, surveillance, diagnosis, and management strategies.                                 | 2024 | R. Katie Morris, Edward Johnstone, Christoph Lees, et al.      | RCOG      |
| Management of refractory overactive bladder                                                                            | The article discusses the management of refractory overactive bladder, focusing on the efficacy and safety of treatments like botulinum toxin, sacral nerve stimulation, and percutaneous tibial nerve stimulation.                                                            | 2016 | Julie Wong, Douglas G Tincello                                 | TOG       |
| Postnatal care                                                                                                         | This guideline covers the routine postnatal care that women and their babies should receive in the first 8 weeks after birth, including the organisation and delivery of care, identifying and managing health problems, and supporting baby feeding and emotional attachment. | 2021 | –                                                              | NICE      |
| Pregnancy in underweight women: implications, management and outcomes                                                  | This article explores the implications, management, and outcomes of pregnancy in underweight women, highlighting the lack of evidence-based guidance and the need for individualized care.                                                                                     | 2022 | Robert Burnie, Edward Golob, Sonji Clarke                      | TOG       |
| Diagnostic Laparoscopy                                                                                                 | This guidance provides advice for clinicians on obtaining consent from women undergoing diagnostic laparoscopy, ensuring consistent and adequate information is given for informed consent.                                                                                    | 2017 | Mr S Banerjee FRCOG, Mr KS Arambage MSc, MRCOG, et al.         | RCOG      |
| Domestic violence: a neglected epidemic in obstetrics and gynaecology training                                         | The article discusses the need for improved education on domestic violence in obstetrics and gynaecology training, highlighting its impact on maternal and fetal health and advocating for its inclusion in medical curricula.                                                 | 2017 | Chantal Cox-George, Joanne Moffatt, Kevin Jones                | TOG       |
| Obstetric and perinatal outcomes in women with endometriosis                                                           | This article reviews the impact of endometriosis on obstetric and perinatal outcomes, highlighting increased risks of complications such as miscarriage, pre-eclampsia, and preterm birth.                                                                                     | 2022 | Junaid Rafi, P. D. M. Pathiraja, Emily Gelson, et al.          | TOG       |
| Imaging in pregnancy                                                                                                   | The article reviews the safety, risks, and benefits of various imaging modalities in pregnancy, emphasizing the importance of appropriate imaging techniques for diagnosing common medical symptoms in pregnant women.                                                         | 2019 | Kelly-Ann Eastwood, Aarthi R Mohan                             | TOG       |
| The Management of Nausea and Vomiting in Pregnancy and Hyperemesis Gravidarum (Green-top Guideline No. 69)             | This guideline provides updated evidence-based recommendations for the diagnosis and management of nausea and vomiting in pregnancy (NVP) and hyperemesis gravidarum (HG), emphasizing the use of validated assessment tools and appropriate pharmacological treatments.       | –    | Catherine Nelson-Piercy, Caitlin Dean, Manjeet Shehmar, et al. | RCOG      |
| Prevention of Early-onset Neonatal Group B Streptococcal Disease                                                       | This guideline provides recommendations for the prevention of early-onset neonatal group B streptococcal disease, including antenatal screening, intrapartum antibiotic prophylaxis, and management strategies for at-risk pregnancies.                                        | 2017 | Hughes RG, Brocklehurst P, Steer PJ, et al.                    | RCOG      |

Continued on next page

Table 1 – continued from previous page

| Title                                                                                                                     | Synopsis                                                                                                                                                                                                                                                                               | Year | Authors                                                           | Publisher                       |
|---------------------------------------------------------------------------------------------------------------------------|----------------------------------------------------------------------------------------------------------------------------------------------------------------------------------------------------------------------------------------------------------------------------------------|------|-------------------------------------------------------------------|---------------------------------|
| Robotic surgery in gynaecology                                                                                            | The paper discusses the use of robotic-assisted keyhole surgery in gynaecology, highlighting its benefits in surgical performance, reduced complications, and improved ergonomics for surgeons, while addressing the higher costs associated with the technology.                      | 2022 | Marielle A. E. Nobbenhuis, Nahid Gul, Peter Barton-Smith, et al.  | RCOG                            |
| The perforated uterus                                                                                                     | The article discusses the risks, prevention, and management of uterine perforation, a rare but serious complication in gynecological procedures.                                                                                                                                       | 2013 | Fevzi Shakir, Yasser Diab                                         | TOG                             |
| Assisted Vaginal Birth                                                                                                    | This guideline provides evidence-based recommendations on the use of forceps and vacuum extraction for assisted vaginal births, aiming to ensure safe clinical practice and effective communication.                                                                                   | 2020 | DJ Murphy, BK Strachan, R Bahl                                    | RCOG                            |
| Endometriosis: diagnosis and management                                                                                   | This guideline covers diagnosing and managing endometriosis, including where fertility is a priority, aiming to raise awareness of symptoms and provide clear advice on referral, diagnosis, and treatment options.                                                                    | 2024 | –                                                                 | NICE                            |
| REGISTRATION OF STILLBIRTHS AND CERTIFICATION FOR PREGNANCY LOSS BEFORE 24 WEEKS OF GESTATION                             | The document provides guidance on the interpretation and implementation of the law regarding the registration of stillbirths and certification for pregnancy loss before 24 weeks of gestation.                                                                                        | 2004 | –                                                                 | RCOG                            |
| Opioid misuse in pregnancy                                                                                                | This article provides an overview of the effects of opioid misuse in pregnancy and helps readers to develop strategies for delivering effective care and minimising harm for this vulnerable and high-risk group.                                                                      | 2022 | Sara Thomson, Ahmed Khalil, Sadie Hafford, et al.                 | TOG                             |
| British HIV Association guidelines for the management of HIV in pregnancy and postpartum 2018 (2020 third interim update) | The guidelines provide comprehensive recommendations for the management of HIV in pregnant and postpartum women, focusing on antiretroviral therapy, prevention of vertical transmission, and specific considerations for co-infections and psychosocial care.                         | 2020 | Dr Yvonne Gilleece, Dr Shema Tariq, Ms Funmi Awosusi, et al.      | British HIV Association (BHIVA) |
| Diabetes in pregnancy: management from preconception to the postnatal period                                              | This guideline covers managing diabetes and its complications in women who are planning pregnancy or are already pregnant, aiming to improve the diagnosis of gestational diabetes and help women with diabetes to self-manage their blood glucose levels before and during pregnancy. | 2015 | –                                                                 | NICE                            |
| Manual vacuum aspiration: an outpatient alternative for surgical management of miscarriage                                | Manual vacuum aspiration (MVA) is a safe and effective alternative to electric vacuum aspiration for surgical management of miscarriage, offering benefits such as reduced waiting time, cost, and avoidance of general anaesthesia.                                                   | 2015 | Mona Sharma                                                       | TOG                             |
| Care in pregnancies subsequent to stillbirth or perinatal death                                                           | The article discusses the increased risks and necessary care strategies for pregnancies following a stillbirth, highlighting the importance of multidisciplinary care and psychological support for parents.                                                                           | 2020 | Nicole Graham, Louise Stephens, Alexander EP Heazell              | TOG                             |
| 'It takes a village' – fertility treatment using donor gametes, embryos and/or surrogacy                                  | The article discusses the increasing use of donor gametes, embryos, and surrogacy in fertility treatments, highlighting clinical indications, ethical and legal implications, and treatment outcomes.                                                                                  | 2022 | Claudia Raperport, Elpiniki Chronopoulou, Anna McLaughlin, et al. | TOG                             |

Continued on next page

Table 1 – continued from previous page

| Title                                                                                                                 | Synopsis                                                                                                                                                                                                                                                                          | Year | Authors                                                                       | Publisher |
|-----------------------------------------------------------------------------------------------------------------------|-----------------------------------------------------------------------------------------------------------------------------------------------------------------------------------------------------------------------------------------------------------------------------------|------|-------------------------------------------------------------------------------|-----------|
| Ultrasound from Conception to 10+0 Weeks of Gestation                                                                 | This paper addresses the safety and application of ultrasound during the embryonic period, focusing on medical and nonmedical uses and the potential risks and benefits.                                                                                                          | 2015 | Mr C Lees, Professor J Abramowicz, Professor C Brezinka, et al.               | RCOG      |
| AMNIOCENTESIS                                                                                                         | This paper provides advice for clinicians on obtaining consent for women undergoing amniocentesis, ensuring consistent and adequate information for valid consent.                                                                                                                | 2005 | Dr AD Cameron<br>FRCOG, Glasgow                                               | RCOG      |
| Insulin pumps and pregnancy                                                                                           | The article discusses the use of insulin pumps in managing diabetes during pregnancy, highlighting their benefits, challenges, and future potential.                                                                                                                              | 2016 | Sara L White,<br>Anna Brackenridge,<br>Daghi Rajasingam                       | TOG       |
| The obstetrician's role in preventing cardiometabolic disease                                                         | This article discusses the role of obstetricians in preventing cardiometabolic diseases by identifying at-risk women during pregnancy and integrating preventive care into maternity services.                                                                                    | 2019 | Jane Elizabeth Hirst,<br>Shobhana Nagraj,<br>Amanda Henry, et al.             | TOG       |
| Urinary tract injuries in laparoscopic gynaecological surgery; prevention, recognition and management                 | This article reviews the incidence, prevention, recognition, and management of urinary tract injuries during laparoscopic gynaecological surgery.                                                                                                                                 | 2014 | Vasileios Minas,<br>Nahid Gul, Thomas Aust, et al.                            | TOG       |
| Detecting endometrial cancer                                                                                          | The article discusses the detection of endometrial cancer, highlighting current diagnostic pathways, risk factors, and the development of novel detection tools.                                                                                                                  | 2021 | Eleanor R Jones,<br>Helena O'Flynn,<br>Kelechi Njoku, et al.                  | TOG       |
| Air Travel and Pregnancy                                                                                              | This paper provides guidance on the suitability of air travel for pregnant women, addressing physiological and environmental changes, potential risks, and practical advice for safe travel.                                                                                      | 2013 | Professor I Greer<br>FRCOG, Liverpool                                         | RCOG      |
| Targeted Therapies for the Management of Ovarian Cancer                                                               | This paper discusses the development and evaluation of targeted therapies for ovarian cancer, focusing on angiogenesis inhibitors and PARP inhibitors, and highlights the challenges and potential of these treatments.                                                           | 2013 | Dr S Banerjee<br>MBBS MA MRCP<br>PhD, Professor M<br>Gore MBBS PhD<br>FRCP    | RCOG      |
| Antenatal corticosteroids to reduce neonatal morbidity and mortality                                                  | This guideline provides evidence-based recommendations on the use of antenatal corticosteroids to improve neonatal outcomes in women at risk of preterm birth or undergoing caesarean birth at term.                                                                              | 2022 | SJ Stock, AJ Thomson,<br>S Papworth                                           | RCOG      |
| Information sharing and communication in management of large for gestational age (LGA) babies in non-diabetic mothers | The article discusses the challenges and importance of information sharing and communication in managing large for gestational age (LGA) babies in non-diabetic mothers, highlighting the lack of specific guidelines and the need for shared decision-making tools.              | 2023 | Gurnaaz Kahlon,<br>Sophie Relph, Wai<br>Yoong                                 | TOG       |
| Management of Gestational Trophoblastic Disease                                                                       | This guideline provides comprehensive information on the presentation, diagnosis, management, treatment, and follow-up of gestational trophoblastic disease (GTD) and gestational trophoblastic neoplasia (GTN), including advice on future pregnancy outcomes and contraception. | 2021 | Tidy J, Seckl M,<br>Hancock BW                                                | RCOG      |
| Understanding precocious puberty in girls                                                                             | This article discusses the definition, causes, evaluation, and treatment of precocious puberty in girls, highlighting the importance of understanding normal pubertal development and the role of gonadotrophin-releasing hormone analogues in treatment.                         | 2012 | Sakunthala Sahithi<br>Tirumuru, Prati-<br>bha Arya, Pallavi<br>Latthe, et al. | TOG       |
| Litigation in gynaecology                                                                                             | The article discusses the reasons for litigation in gynaecology, the anatomy of a claim, and strategies to avoid litigation, highlighting key medico-legal rulings and ethical issues.                                                                                            | 2014 | Swati Jha, Sarah<br>Rowland                                                   | TOG       |

Continued on next page

Table 1 – continued from previous page

| Title                                                                                                                 | Synopsis                                                                                                                                                                                                                                                                                                                              | Year | Authors                                                               | Publisher   |
|-----------------------------------------------------------------------------------------------------------------------|---------------------------------------------------------------------------------------------------------------------------------------------------------------------------------------------------------------------------------------------------------------------------------------------------------------------------------------|------|-----------------------------------------------------------------------|-------------|
| The role of thrombophilia testing in women with adverse pregnancy outcomes                                            | This article critically evaluates the benefit of thrombophilia testing in the obstetric setting and provides guidance on the care of women in subsequent pregnancies following adverse outcomes.                                                                                                                                      | 2017 | Julia Unterscheider, Stefan C Kane, Briony Cutts, et al.              | TOG         |
| Antenatal and postnatal mental health: clinical management and service guidance                                       | This guideline covers recognising, assessing, and treating mental health problems in women who are planning to have a baby, are pregnant, or have had a baby or been pregnant in the past year, promoting early detection and good management to improve women's quality of life during pregnancy and in the year after giving birth. | 2014 | –                                                                     | NICE        |
| Perioperative management of women on oral anticoagulants and antiplatelet agents undergoing gynaecological procedures | This article provides guidance on managing women on oral anticoagulants and antiplatelet agents who require elective and emergency gynaecological procedures, emphasizing the importance of individualized care and collaboration with haematologists.                                                                                | 2020 | Edwina Goh, Victoria Barker, Pei Ling Lee, et al.                     | TOG         |
| Intrahepatic cholestasis of pregnancy                                                                                 | This article reviews the presentation, investigation, and management of intrahepatic cholestasis of pregnancy (ICP), highlighting its associated risks and treatment options.                                                                                                                                                         | 2016 | Victoria Geenes, Catherine Williamson, Lucy C Chappell                | TOG         |
| Postpartum perineal wound dehiscence                                                                                  | This article reviews perineal wound dehiscence, its risk factors, management strategies, and the benefits of surgical intervention over conservative treatment.                                                                                                                                                                       | 2023 | Tarek El Shamy, Eleanor Sein, Sunita Sharma, et al.                   | TOG         |
| Vaginal estrogen deficiency                                                                                           | The article discusses the causes, symptoms, and treatment options for vaginal estrogen deficiency, particularly in postmenopausal women, highlighting the impact on quality of life and the need for improved management.                                                                                                             | 2019 | Shirin Khanjani, Nick Panay                                           | TOG         |
| The fallopian tube as the origin of non-uterine pelvic high-grade serous carcinoma                                    | This article reviews the evidence suggesting that the fimbrial end of the fallopian tube may be the origin of non-uterine high-grade pelvic serous carcinoma, discusses the clinical management of serous tubal intraepithelial carcinoma (STIC), and explores preventative strategies for high-grade pelvic serous carcinoma.        | 2016 | Ieera Madan Aggarwal, Yu Hui Lim, Timothy Yong Kuei Lim               | TOG         |
| Ovarian cancer: recognition and initial management                                                                    | This guideline covers detecting, diagnosing and treating women who have, or are suspected of having, epithelial ovarian cancer, aiming to enable earlier detection and improve initial treatment.                                                                                                                                     | 2011 | –                                                                     | NICE        |
| Nerve injuries associated with gynaecological surgery                                                                 | This article discusses the common occurrence of nerve injuries during gynaecological surgery, their causes, management, and prevention strategies.                                                                                                                                                                                    | 2014 | Olayemi Kuponiyi, Djavid I Alleemudder, Adeyinka Latunde-Dada, et al. | TOG         |
| Uterine arteriovenous malformations: clinical implications                                                            | The article discusses the incidence, diagnosis, and management of uterine arteriovenous malformations (AVMs), highlighting their clinical implications and treatment options.                                                                                                                                                         | 2015 | Thangamma Katimada Annaiah, Sreejith Kodakkattil Sreenivasan          | TOG         |
| Guidance 3. Providing a quality colposcopy clinic                                                                     | This guidance outlines the standards and protocols for operating a quality-assured colposcopy clinic, including roles, training, and operational procedures.                                                                                                                                                                          | 2024 | –                                                                     | NHS England |
| Extreme prematurity and perinatal management                                                                          | The article discusses the medical and ethical considerations in the perinatal management of pregnant women delivering at the threshold of viability, emphasizing the importance of multidisciplinary advice and parental consensus on optimal care.                                                                                   | 2018 | Anna L David, Aung Soe                                                | TOG         |

Continued on next page

Table 1 – continued from previous page

| Title                                                                                                      | Synopsis                                                                                                                                                                                                                                                                          | Year | Authors                                                | Publisher |
|------------------------------------------------------------------------------------------------------------|-----------------------------------------------------------------------------------------------------------------------------------------------------------------------------------------------------------------------------------------------------------------------------------|------|--------------------------------------------------------|-----------|
| A review of acupuncture in obstetrics and gynaecology                                                      | This article reviews the use of acupuncture in obstetrics and gynaecology, discussing its effectiveness and safety in various conditions such as pain management, fertility, and pregnancy-related issues.                                                                        | 2019 | Faisal Karim, James Dilley, Elaine Cheung              | TOG       |
| Management of palpitations and cardiac arrhythmias in pregnancy                                            | The article discusses the management of palpitations and cardiac arrhythmias in pregnant women, emphasizing the importance of distinguishing between physiological changes and pathological arrhythmias, and the safe use of anti-arrhythmic treatments during pregnancy.         | 2019 | Anna Roberts, Joseph Mechery, Anthony Mechery, et al.  | TOG       |
| The transgender population: improving awareness for gynaecologists and their role in the provision of care | This article aims to educate gynaecologists on the care required for transgender individuals, emphasizing the importance of understanding the transition process and the role of gynaecologists in providing comprehensive care.                                                  | 2019 | Suzanne Price, Joanne McManus, James Barrett           | TOG       |
| Education The teacher, the learner and the method                                                          | The article discusses the roles and methods of teaching in obstetrics and gynaecology, emphasizing the importance of effective teaching strategies and the attributes of good teachers and learners.                                                                              | 2010 | S J Duthie, A S Garden                                 | TOG       |
| Decision-making framework in gynaecology for patients who lack mental capacity                             | This article explores clinical decision making in gynaecology for individuals who lack independent decision-making ability, emphasizing the importance of the Mental Capacity Act (MCA) 2005 and its best interests principles.                                                   | 2018 | Ibrahim I Bolaji, Edwin Omih, Ka Yan Shirley SZE       | TOG       |
| Elective Egg Freezing for Non-Medical Reasons                                                              | The paper discusses the increasing trend of elective egg freezing for non-medical reasons, highlighting the technological advancements, ethical considerations, and the need for better public education on fertility decline with age.                                           | 2020 | RA Anderson, MC Davies, SA Lavery                      | RCOG      |
| Management of endometriosis-related pelvic pain                                                            | The article discusses the challenges and strategies in diagnosing and managing endometriosis-related pelvic pain, including medical and surgical treatment options.                                                                                                               | 2017 | Wee-Liak Hoo, Rebecca Hardcastle, Keith Louden         | TOG       |
| Antenatal management of singleton pregnancies conceived using assisted reproductive technology             | This article discusses the antenatal management of singleton pregnancies conceived through assisted reproductive technology (ART), highlighting the increased risks of maternal and fetal complications and the importance of understanding these risks for effective monitoring. | 2020 | Alison Richardson, Myles Taylor, Joo P Teoh, et al.    | TOG       |
| –                                                                                                          | The article discusses the prevalence, contributory factors, and effects of burnout among doctors, particularly in the field of obstetrics and gynaecology, and suggests strategies for prevention and management at various levels.                                               | 2019 | Katie Cresswell, Radha Graham, Alison Wright, et al.   | TOG       |
| The role of frozen-thawed embryo replacement cycles in assisted conception                                 | This article explores the rise in frozen-thawed embryo replacement (FER) cycles in assisted conception, highlighting improved outcomes due to advancements in embryo cryopreservation techniques and discussing the implications for IVF practice.                                | 2020 | Matt Noble, Tim Child                                  | TOG       |
| Postural tachycardia syndrome and pregnancy                                                                | This article discusses the challenges and management of postural tachycardia syndrome (PoTS) during pregnancy, highlighting the importance of correct diagnosis and a multidisciplinary approach for optimal outcomes.                                                            | 2018 | Meena Bhatia, Lesley Kavi, Catherine Nelson-Piercy     | TOG       |
| Recurrent Miscarriage                                                                                      | This guideline provides recommendations for the investigation and treatment of recurrent miscarriage, defined as three or more first trimester miscarriages, and includes testing for thrombophilia, genetic factors, and anatomical assessments.                                 | 2023 | Lesley Regan, Rajendra Rai, Sotirios Saravelos, et al. | RCOG      |

Continued on next page

Table 1 – continued from previous page

| Title                                                                       | Synopsis                                                                                                                                                                                                                                                               | Year | Authors                                                                                 | Publisher                                        |
|-----------------------------------------------------------------------------|------------------------------------------------------------------------------------------------------------------------------------------------------------------------------------------------------------------------------------------------------------------------|------|-----------------------------------------------------------------------------------------|--------------------------------------------------|
| The management of pregnancy after trachelectomy for early cervical cancer   | This article discusses the management of pregnancies following trachelectomy for early cervical cancer, highlighting the associated risks and providing guidance for obstetric care.                                                                                   | 2017 | Anushka Tirlapur, Fredric Willmott, Philippa Lloyd, et al.                              | TOG                                              |
| Perinatal Management of Extreme Preterm Birth before 27 weeks of gestation  | This framework provides guidance for the management of extremely preterm births before 27 weeks of gestation, emphasizing a risk-based approach to decision-making and the importance of involving parents in the care process.                                        | 2019 | Dr Sarah E Bates, Ms Erica Everett, Dr Tracey Johnston, et al.                          | British Association of Perinatal Medicine (BAPM) |
| Vulval disorders in paediatric and adolescent patients and their management | This article reviews common vulval disorders in paediatric and adolescent patients, focusing on their presentation, diagnosis, and management, with an emphasis on conservative treatment approaches.                                                                  | 2023 | Salwa Abdullahi Idle, Helen Coles, Jemma Johns                                          | TOG                                              |
| Progress in Cervical Screening in the UK                                    | This paper discusses the developments and challenges in cervical screening in the UK, focusing on the role of HPV in prevention and the impact of HPV vaccination.                                                                                                     | 2016 | Dr TBR Freeman-Wang MRCOG, Professor ME Cruickshank FRCOG, Professor HC Kitchener FRCOG | RCOG                                             |
| Manchester repair ('Fothergill's operation') revisited                      | The article discusses the Manchester repair, a uterus-preserving surgical technique for uterine prolapse, highlighting its indications, procedure, and outcomes compared to vaginal hysterectomy.                                                                      | 2021 | Dhanuson Dharmasena, Clive Spence-Jones, Rajvinder Khasriya, et al.                     | TOG                                              |
| Non-immune hydrops fetalis: a practical guide for obstetricians             | This article provides a practical, evidence-based guide for obstetricians on the evaluation and management of non-immune hydrops fetalis (NIHF), emphasizing the importance of identifying causes antenatally to optimize management and discussing treatment options. | 2023 | Delima Khairudin, Zarko Alfrevic, Fionnuala Mone, et al.                                | TOG                                              |
| The Initial Management of Chronic Pelvic Pain                               | This guideline provides an evidence-based framework for the initial assessment and management of women presenting with chronic pelvic pain.                                                                                                                            | 2012 | Ms SJ Moore MRCOG, Mr SH Kennedy MRCOG                                                  | RCOG                                             |
| Polycystic ovary syndrome (PCOS)                                            | The article discusses the symptoms, diagnosis, management, and implications of polycystic ovary syndrome (PCOS), highlighting its impact on fertility, metabolic health, and quality of life.                                                                          | 2017 | Adam H Balen                                                                            | TOG                                              |
| Update on radiotherapy in gynaecological malignancies                       | This article reviews the evolving role of adjuvant radiation therapy in gynaecological cancer, highlighting recent clinical trials and technological advancements that improve treatment delivery and outcomes.                                                        | 2017 | Nicholas S Reed, Azmat H Sadozye                                                        | TOG                                              |
| Long-term Consequences of Polycystic Ovary Syndrome                         | This guideline provides information to assist clinicians in advising women with polycystic ovary syndrome (PCOS) about the long-term health consequences of the syndrome.                                                                                              | 2014 | Professor WL Ledger, Professor SL Atkin, Dr T Sathyapalan                               | RCOG                                             |
| Guidance 6. Screening and management of immunosuppressed individuals        | This guidance provides updated protocols for the screening and management of immunosuppressed individuals, including those with renal failure, post-transplantation, and HIV, emphasizing the importance of cervical screening and tailored management strategies.     | 2024 | -                                                                                       | NHS England                                      |
| Antenatal and Postnatal Analgesia                                           | This paper clarifies advice regarding pain relief during and after pregnancy, emphasizing the importance of correct analgesic management to minimize risks to mothers and infants.                                                                                     | 2018 | DL Bisson, SD Newell, C Laxton                                                          | RCOG                                             |
| The role of antenatal corticosteroids in improving neonatal outcomes        | This article discusses the use of antenatal corticosteroids (ACS) to reduce neonatal morbidity and mortality, highlighting the challenges of timing, the role of repeat courses, and the need for further research on long-term impacts.                               | 2021 | Paula Busuulwa, Katie Groom, Lucy C Chappell, et al.                                    | TOG                                              |

Continued on next page

Table 1 – continued from previous page

| Title                                                                                                  | Synopsis                                                                                                                                                                                                                                                                                        | Year | Authors                                                                        | Publisher |
|--------------------------------------------------------------------------------------------------------|-------------------------------------------------------------------------------------------------------------------------------------------------------------------------------------------------------------------------------------------------------------------------------------------------|------|--------------------------------------------------------------------------------|-----------|
| Developing situational awareness ('helicopter view')                                                   | The article discusses the importance of situational awareness in clinical practice, highlighting how it can be lost and providing practical tips to maintain it.                                                                                                                                | 2021 | Wai Yoong, Sayantana Patra-Das, Neil Jeffers, et al.                           | TOG       |
| Management of Monochorionic Twin Pregnancy                                                             | This guideline provides recommendations for the management of monochorionic twin pregnancies, focusing on diagnosis, screening, and treatment of associated complications.                                                                                                                      | 2016 | Kilby MD, Bricker L                                                            | RCOG      |
| Update on recurrent vulvovaginal candidiasis                                                           | This article reviews the current literature on recurrent vulvovaginal candidiasis (RVVC), discussing its prevalence, risk factors, diagnosis, and management strategies, including novel therapies.                                                                                             | 2021 | Amy Borland, Katie Ovens, Ifeoma Offiah, et al.                                | TOG       |
| Very advanced maternal age                                                                             | The article discusses the implications, risks, and management strategies for pregnancies in women of very advanced maternal age, particularly those aged 45 years and older, highlighting the increased risks associated with assisted reproductive technologies and multiple pregnancies.      | 2021 | Alice Howell, Margaret Blott                                                   | TOG       |
| Epigenetics and Reproductive Medicine                                                                  | This paper reviews the current understanding of epigenetics in reproductive medicine, focusing on the implications of assisted reproductive technologies on epigenetic changes and their potential long-term effects.                                                                           | 2018 | J Huntriss, AH Balen, KD Sinclair, et al.                                      | RCOG      |
| Fertility problems: assessment and treatment                                                           | This guideline covers diagnosing and treating fertility problems, aiming to reduce variation in practice and improve the management of fertility issues.                                                                                                                                        | 2013 | –                                                                              | NICE      |
| Metabolic syndrome in women with polycystic ovary syndrome                                             | This article reviews the pathogenesis, consequences, diagnostic criteria, screening, and management of metabolic syndrome in women with polycystic ovary syndrome (PCOS).                                                                                                                       | 2018 | Swaramya Chandrasekaran, Haritha Sagili                                        | TOG       |
| Haemoglobinopathy: considerations for reproductive health                                              | This article reviews the impact of iron overload secondary to haemoglobinopathies on reproductive health and discusses current management options for patients with hypogonadotropic hypogonadism due to iron overload.                                                                         | 2018 | Prasanna Raj Supramaniam, Monica Mittal, Deborah Hay, et al.                   | TOG       |
| Current management of recurrent pregnancy loss                                                         | The article provides a systematic and evidence-based evaluation of the current management of recurrent pregnancy loss, highlighting the lack of consensus on definitions, the limited quality of evidence, and the controversies surrounding recommendations for investigations and management. | 2022 | Mark R Chester, Anushka Tirilapur, Kanna Jayaprakasan                          | TOG       |
| Diagnosis and management of tubo-ovarian abscesses                                                     | This article discusses the diagnosis and management strategies for tubo-ovarian abscesses, a severe form of pelvic inflammatory disease, highlighting the importance of prompt treatment to prevent complications such as infertility and chronic pelvic pain.                                  | 2018 | Kirsty Munro, Asma Gharaibeh, Sangeetha Nagabushanam, et al.                   | TOG       |
| Hysteroscopic mechanical tissue removal (hysteroscopic morcellation) for uterine fibroids              | This guidance by NICE discusses the safety, efficacy, and procedural considerations for hysteroscopic mechanical tissue removal of uterine fibroids, recommending its use with special clinical arrangements due to potential risks and limited evidence.                                       | 2021 | –                                                                              | NICE      |
| Clinical recommendations on the use of uterine artery embolisation (UAE) in the management of fibroids | This publication provides clinical recommendations and guidelines for the use of uterine artery embolisation (UAE) in the management of fibroids, highlighting its efficacy, safety, and considerations for patient care.                                                                       | 2013 | Dr Christopher Hammond, Dr Tony Nicholson, Professor Anthony Watkinson, et al. | RCOG      |

Continued on next page

Table 1 – continued from previous page

| Title                                                                                                 | Synopsis                                                                                                                                                                                                                                             | Year | Authors                                                            | Publisher                                                             |
|-------------------------------------------------------------------------------------------------------|------------------------------------------------------------------------------------------------------------------------------------------------------------------------------------------------------------------------------------------------------|------|--------------------------------------------------------------------|-----------------------------------------------------------------------|
| Endometriosis                                                                                         | The guideline provides clinical recommendations for the diagnosis and treatment of endometriosis to improve healthcare delivery in the field of human reproduction and embryology.                                                                   | –    | –                                                                  | European Society of Human Reproduction and Embryology (ESHRE)<br>RCOG |
| Care of Women with Obesity in Pregnancy                                                               | This guideline provides comprehensive recommendations for the care of pregnant women with obesity, covering preconception, antenatal, and postnatal care, and addressing the associated risks and management strategies.                             | 2018 | Denison FC, Aedla NR, Keag O, et al.                               | RCOG                                                                  |
| Saving Lives, Improving Mothers' Care                                                                 | This report presents lessons learned to inform maternity care from the UK and Ireland Confidential Enquiries into Maternal Deaths and Morbidity between 2020 and 2022.                                                                               | 2024 | Allison Felker, Roshni Patel, Rohit Kotnis, et al.                 | NPEU, Univ. Oxford                                                    |
| External Cephalic Version and Reducing the Incidence of Term Breech Presentation                      | This guideline describes and summarises the best evidence concerning methods to prevent non-cephalic presentation at delivery and therefore, caesarean section and its sequelae.                                                                     | 2017 | Impey LWM, Murphy DJ, Griffiths M, et al.                          | RCOG                                                                  |
| The Effect of Surgery for Endometriomas on Fertility                                                  | This Scientific Impact Paper reviews the current evidence for the management of endometriomas within the context of infertility treatment, discussing the potential impacts of surgery on fertility and ovarian reserve.                             | 2017 | K Jayaprakasan, C Becker, M Mittal                                 | RCOG                                                                  |
| The molecular and genetic basis of inherited cancer risk in gynaecology                               | This article explores the genetic mutations associated with hereditary gynaecological cancers, focusing on the Fanconi Anaemia-BRCA pathway and other genetic factors influencing cancer risk.                                                       | 2015 | James P Beirne, Gareth W Irwin, Stuart A McIntosh, et al.          | TOG                                                                   |
| Prenatal genomic testing for ultrasound-detected fetal structural anomalies                           | The article discusses various genomic testing strategies for diagnosing fetal structural anomalies detected via ultrasound, highlighting the benefits, challenges, and ethical considerations of these technologies.                                 | 2023 | Kelly Reilly, Caoimhe McKenna, Simon McCullough, et al.            | TOG                                                                   |
| Management of Endometrial Hyperplasia                                                                 | This guideline provides evidence-based recommendations for the management of endometrial hyperplasia, including classification, diagnostic methods, and treatment options.                                                                           | 2016 | –                                                                  | RCOG                                                                  |
| British Gynaecological Cancer Society (BGCS) Cervical Cancer Guidelines: Recommendations for Practice | The guideline provides evidence-based recommendations for the diagnosis and management of cervical cancer in the UK, covering aspects from screening to advanced disease management.                                                                 | 2020 | Nick Reed, Janos Balega, Tara Barwick, et al.                      | British Gynaecological Cancer Society (BGCS)                          |
| Hypertension in pregnancy: diagnosis and management                                                   | This guideline covers diagnosing and managing hypertension, including pre-eclampsia, during pregnancy, labour, and birth, aiming to improve care for women and their babies.                                                                         | 2019 | –                                                                  | NICE                                                                  |
| Umbilical Cord Blood Banking                                                                          | This paper provides advice on the scientific basis, clinical use, safety, and legal implications of umbilical cord blood storage, distinguishing between personal and altruistic storage, and discusses the future utility of cord blood stem cells. | 2006 | Professor Peter Braude, Dr Susan Bewley, Dr Melanie Davies, et al. | RCOG                                                                  |
| Solid organ transplantation in pregnancy                                                              | This article discusses the management and outcomes of pregnancy in women with solid organ transplants, focusing on renal transplantation and comparing it with other organ transplants.                                                              | 2016 | Kate S Wiles, Alexandra L Tillet, Kate R Harding                   | TOG                                                                   |
| Consent in clinical practice                                                                          | This article reviews best practices for obtaining consent in both elective and emergency medical situations, focusing on legal and ethical considerations in obstetrics and gynaecology.                                                             | 2015 | Alan Treharne, Bryan Beattie                                       | TOG                                                                   |

Continued on next page

Table 1 – continued from previous page

| Title                                                                                                       | Synopsis                                                                                                                                                                                                                                                                                                                              | Year | Authors                                                                        | Publisher |
|-------------------------------------------------------------------------------------------------------------|---------------------------------------------------------------------------------------------------------------------------------------------------------------------------------------------------------------------------------------------------------------------------------------------------------------------------------------|------|--------------------------------------------------------------------------------|-----------|
| Maternal Collapse in Pregnancy and the Puerperium                                                           | This guideline discusses the identification, causes, and management of maternal collapse during pregnancy and the puerperium, emphasizing the importance of prompt and effective resuscitation.                                                                                                                                       | 2020 | J Chu, TA Johnston, J Geoghegan, et al.                                        | BJOG      |
| Polycystic ovary syndrome and the differential diagnosis of hyperandrogenism                                | The article discusses the diagnosis of polycystic ovary syndrome (PCOS) and the differential diagnosis of hyperandrogenism, highlighting the challenges and limitations of biochemical testing for testosterone in women.                                                                                                             | 2013 | Claire L Meek, Vasiliki Bravis, Abigail Don, et al.                            | TOG       |
| Gynaecological morbidity associated with caesarean niche: increasing awareness, prevention and management   | This review discusses the gynaecological morbidity associated with caesarean niche, highlighting the importance of awareness, prevention, and management of this condition.                                                                                                                                                           | 2020 | Adam J Brook, Fiona R Clarke, Kalsang Bhatia                                   | TOG       |
| Reduced Fetal Movements                                                                                     | This guideline provides advice for clinicians on managing women presenting with reduced fetal movements during pregnancy, reviewing risk factors and management recommendations.                                                                                                                                                      | 2011 | Dr MK Whitworth MRCOG, Professor M Fisher, Dr A Heazell MRCOG                  | RCOG      |
| Intrapartum care                                                                                            | This guideline covers the care of women and their babies during labour and immediately after birth, focusing on women who give birth between 37 and 42 weeks of pregnancy, and aims to help women make informed choices about their care and reduce variation in care aspects.                                                        | 2023 | –                                                                              | NICE      |
| The Management of Third- and Fourth-Degree Perineal Tears                                                   | This guideline provides evidence-based recommendations for the diagnosis, management, and treatment of third- and fourth-degree perineal tears, also known as obstetric anal sphincter injuries (OASIS).                                                                                                                              | 2015 | Mr RJ Fernando FRCOG, Mr AH Sultan FRCOG, Professor RM Freeman FRCOG, et al.   | RCOG      |
| Care of Women Presenting with Suspected Preterm Prelabour Rupture of Membranes from 24+0 Weeks of Gestation | The guideline provides recommendations for the diagnosis, assessment, care, and timing of birth for women presenting with suspected preterm prelabour rupture of membranes (PPROM) from 24+0 to 36+6 weeks of gestation.                                                                                                              | 2019 | AJ Thomson, on behalf of the Royal College of Obstetricians and Gynaecologists | BJOG      |
| Antenatal and post-natal mental health: clinical management and service guidance                            | This guideline covers recognising, assessing, and treating mental health problems in women who are planning to have a baby, are pregnant, or have had a baby or been pregnant in the past year, promoting early detection and good management to improve women’s quality of life during pregnancy and in the year after giving birth. | 2014 | –                                                                              | NICE      |
| Multiple sclerosis and pregnancy                                                                            | This article provides an overview of the effects of multiple sclerosis on pregnancy, the impact of pregnancy on the disease, and the safety of medications used during pregnancy and breastfeeding.                                                                                                                                   | 2019 | Priya Kanagaraj, Nikos Evangelou, Dipanwita Kapoor                             | TOG       |
| Issues around vaginal vault closure                                                                         | The article reviews various techniques for vaginal vault closure post-hysterectomy, discussing their advantages, disadvantages, and associated complications.                                                                                                                                                                         | 2019 | Magdy Moustafa, Mohamed Elnasharty                                             | TOG       |
| Management of Bartholin’s cyst and abscess                                                                  | This article discusses the management strategies for Bartholin’s cyst and abscess, including conservative and surgical options, with a focus on outpatient procedures like the balloon Word catheter.                                                                                                                                 | 2023 | Ayesha Paracha, Bati-Mona Sharma                                               | TOG       |
| Biologics in pregnancy – for the obstetrician                                                               | The article discusses the use of biologics during pregnancy, their potential side effects, and the importance of individualized treatment plans to manage autoimmune diseases while minimizing risks to the fetus.                                                                                                                    | 2016 | May Ching Soh, Lucy MacKillop                                                  | TOG       |

Continued on next page

Table 1 – continued from previous page

| Title                                                                                                                                                     | Synopsis                                                                                                                                                                                                                                   | Year | Authors                                                    | Publisher   |
|-----------------------------------------------------------------------------------------------------------------------------------------------------------|--------------------------------------------------------------------------------------------------------------------------------------------------------------------------------------------------------------------------------------------|------|------------------------------------------------------------|-------------|
| The prevention of malaria in pregnancy                                                                                                                    | This guideline provides evidence-based information for clinicians on preventing malaria in pregnancy for UK-based residents visiting malaria endemic areas.                                                                                | 2010 | Dr R McGready, Dr EA Ashley, Professor F Nosten, et al.    | RCOG        |
| Update on chemotherapy in gynaecological cancers                                                                                                          | This article reviews the use of chemotherapy in gynaecological cancers, focusing on current therapeutic options and new developments in treatment, particularly for ovarian cancer.                                                        | 2016 | Nicholas S Reed, Azmat H Sadozye                           | TOG         |
| Guidance 1. Introduction and programme policy                                                                                                             | The NHS Cervical Screening Programme aims to reduce cervical cancer incidence and mortality through a systematic, quality-assured screening programme, with updates on primary HPV screening and screening intervals.                      | 2024 | –                                                          | NHS England |
| A practical guide to quality improvement                                                                                                                  | This article provides an overview of quality improvement techniques and methodologies to help clinicians improve healthcare quality, efficiency, and patient experience.                                                                   | 2017 | Susanna Crowe, Sanjula Sharma                              | TOG         |
| The use of biomarkers to stratify surgical care in women with ovarian cancer                                                                              | This paper discusses the potential of biomarkers to personalize surgical care for ovarian cancer, highlighting the need for research to validate biomarkers that can predict surgical outcomes and improve individualized treatment plans. | 2022 | D. L. Phelps, J. V. Borley, R. Brown, et al.               | RCOG        |
| Diagnostic Biomarkers for Predicting Adverse Early Pregnancy Outcomes                                                                                     | This paper discusses the current use and potential future use of biomarkers in predicting adverse early pregnancy outcomes, highlighting the limitations and controversies surrounding existing biomarkers.                                | 2018 | M Memtsa, D Jurkovic, ERM Jauniaux                         | RCOG        |
| A guide to indications, components and interpretation of urodynamic investigations                                                                        | This article provides an overview of the indications, components, and interpretation of urodynamic investigations, emphasizing the importance of accurate diagnosis and management of lower urinary tract symptoms.                        | 2019 | Annika Taithongchai, Abdul H Sultan, Raneer Thakar         | TOG         |
| Vulvodynia: integrating current knowledge into clinical practice                                                                                          | This article provides a comprehensive review of recent terminology, classification, methods of diagnosis, and current evidence-based recommendations in the treatment strategies of vulvodynia.                                            | 2014 | Kavitha Nagandla, Nalliah Sivalingam                       | TOG         |
| Acute and chronic pancreatitis in pregnancy                                                                                                               | The article reviews the diagnosis, causes, and management of acute and chronic pancreatitis in pregnancy, highlighting the challenges and considerations for both maternal and fetal health.                                               | 2021 | Josie L O’Heney, Rebecca E Barnett, Ruth M MacSwan, et al. | TOG         |
| The Combined Use of Ultrasound and Fetal Magnetic Resonance Imaging for a Comprehensive Fetal Neurological Assessment in Fetal Congenital Cardiac Defects | This paper discusses the use of ultrasound and MRI in assessing fetal brain development in cases of congenital cardiac defects, highlighting the potential for improved diagnosis and counselling regarding neurodevelopmental outcomes.   | 2019 | D Pasupathy, ML Denbow, MA Rutherford                      | RCOG        |
| Continence surgery at the time of pelvic organ prolapse repair: a review of the literature                                                                | This article reviews the current literature on surgical treatment for concomitant stress urinary incontinence and pelvic organ prolapse surgery, discussing the benefits and challenges of combined versus staged surgical approaches.     | 2019 | Jemina Loganathan, Abdalla Fayyad, Mohamed Abdel-Fattah    | TOG         |
| The role of ultrasonography in the diagnosis and management of early pregnancy complications                                                              | This article reviews the pivotal role of ultrasonography in diagnosing and managing early pregnancy complications, emphasizing the importance of accurate diagnosis to prevent misdiagnosis and inappropriate treatment.                   | 2015 | Maya Al-Memar, Emma Kirk, Tom Bourne                       | TOG         |

Continued on next page

Table 1 – continued from previous page

| Title                                                                                      | Synopsis                                                                                                                                                                                                                                                       | Year | Authors                                                                                | Publisher |
|--------------------------------------------------------------------------------------------|----------------------------------------------------------------------------------------------------------------------------------------------------------------------------------------------------------------------------------------------------------------|------|----------------------------------------------------------------------------------------|-----------|
| Antenatal and intrapartum care of pregnancy complicated by lethal fetal anomaly            | The article discusses the management of pregnancies complicated by lethal fetal anomalies, emphasizing the importance of a multidisciplinary approach to address the medical, emotional, and spiritual needs of affected families.                             | 2013 | Karen McNamara, Keelin O'Donoghue, Orla O'Connell, et al.                              | TOG       |
| Management of term breech presentation                                                     | This article provides an update on the management of breech presentation at term, focusing on vaginal breech birth and discussing the evidence, challenges, and recommendations for practice.                                                                  | 2023 | Paul Timmons, Victoria Wallis, Shawn Walker, et al.                                    | TOG       |
| Antepartum Haemorrhage                                                                     | This guideline addresses the management of antepartum haemorrhage (APH), a significant cause of maternal and perinatal morbidity and mortality, focusing on its causes, risk factors, and management strategies.                                               | 2011 | –                                                                                      | RCOG      |
| Surgical management of bowel obstruction in gynaecological cancer                          | The article discusses the complexities and considerations in managing bowel obstruction in women with gynaecological cancer, emphasizing the need for a multidisciplinary approach and highlighting the challenges in surgical and non-surgical interventions. | 2017 | Desiree F Kolumainen, Julia Riley, Jayne Wood, et al.                                  | TOG       |
| Networked maternal medicine services in England and the role of the obstetric physician    | The article discusses the development and implementation of networked maternal medicine services in England, emphasizing the role of obstetric physicians in improving care for pregnant women with medical conditions.                                        | 2021 | Lucy Mackillop                                                                         | TOG       |
| Advances and applications in fetal magnetic resonance imaging                              | This article describes recent advances in fetal MRI, focusing on overcoming challenges related to fetal motion, and discusses current clinical applications and imaging techniques that complement ultrasound.                                                 | 2015 | Lisa Story, Mary Rutherford                                                            | TOG       |
| Ectopic pregnancy and miscarriage: diagnosis and initial management                        | This guideline covers diagnosing and managing ectopic pregnancy and miscarriage in women with complications in early pregnancy, aiming to improve diagnosis and support to limit psychological impact.                                                         | 2019 | –                                                                                      | NICE      |
| Developing New Pharmaceutical Treatments for Obstetric Conditions                          | This paper discusses the challenges in developing therapeutics in obstetrics and identifying best practices.                                                                                                                                                   | 2015 | Dr AL David MRCOG, Professor S Thornton FRCOG, Dr A Sutcliffe MD PhD PG Dip CT, et al. | RCOG      |
| Evolution in screening for Down syndrome                                                   | This article describes the evolution of screening methods for fetal trisomy 21, highlighting advancements from maternal age-based screening to cell-free DNA analysis, which offers a 99% detection rate with a 0.1% false positive rate.                      | 2019 | Ghalia Ashoor Al Mahri, KH Nicolaidis                                                  | TOG       |
| Reducing the Risk of Venous Thromboembolism during Pregnancy and the Puerperium            | This guideline provides advice on the prevention of venous thromboembolism (VTE) during pregnancy, birth, and following delivery, emphasizing risk assessment and management strategies.                                                                       | 2015 | –                                                                                      | RCOG      |
| Consenting, competence and confidentiality in paediatric adolescent gynaecology            | This article addresses the legal and ethical principles of consent, competence, and confidentiality in paediatric adolescent gynaecology, highlighting the challenges and guidelines for healthcare professionals in the UK.                                   | 2023 | RN Pillai, M Narayanan, M Choudhary                                                    | TOG       |
| Ocular manifestations of pregnancy and labour: from the innocuous to the sight threatening | This article explores the various ocular changes that can occur during pregnancy, ranging from harmless physiological changes to serious sight-threatening conditions, and discusses appropriate management and referral pathways.                             | 2020 | Ajay D Patil, Abdallah A Ellabban, Dilip B Patil, et al.                               | TOG       |

Continued on next page

Table 1 – continued from previous page

| Title                                                                                                                 | Synopsis                                                                                                                                                                                                                                                                                                                                                      | Year | Authors                                                                             | Publisher                                                                   |
|-----------------------------------------------------------------------------------------------------------------------|---------------------------------------------------------------------------------------------------------------------------------------------------------------------------------------------------------------------------------------------------------------------------------------------------------------------------------------------------------------|------|-------------------------------------------------------------------------------------|-----------------------------------------------------------------------------|
| Gastrointestinal congenital anomalies requiring surgery: diagnosis, counselling, and management                       | This article reviews the diagnosis, counselling, and management of gastrointestinal congenital anomalies requiring surgery, emphasizing the importance of multidisciplinary team management in fetal medicine.                                                                                                                                                | 2023 | Stuart Mires, Arun Raychoudhury, Timothy Overton, et al.                            | TOG                                                                         |
| British Gynaecological Cancer Society (BGCS) vulval cancer guidelines: An update on recommendations for practice 2023 | This publication provides updated evidence-based guidelines for the management and diagnosis of vulval carcinoma, focusing on recommendations for healthcare professionals treating vulval cancer and related conditions.                                                                                                                                     | 2023 | Jo Morrison, Peter Baldwin, Louise Hanna, et al.                                    | European Journal of Obstetrics & Gynecology and Reproductive Biology<br>TOG |
| An update on the management of male infertility                                                                       | This article reviews the current state of male infertility management, focusing on lifestyle factors, sperm assessment, selection tests, and genetic testing, while highlighting the need for further research and ethical considerations in treatment.                                                                                                       | 2020 | Stamatios Karavolos, Nikolett Panagiotopoulou, Hisham Alahwany, et al.              | TOG                                                                         |
| Cervical Cerclage                                                                                                     | This guideline provides evidence-based recommendations on the use of cervical cerclage in women at risk of preterm birth and second trimester loss, supplementing NICE guideline NG25.                                                                                                                                                                        | 2022 | AH Shennan, L Story on behalf of the Royal College of Obstetricians, Gynaecologists | BJOG                                                                        |
| Postpartum ovarian vein thrombosis                                                                                    | The article discusses the rare but potentially fatal condition of postpartum ovarian vein thrombosis (POVT), its symptoms, diagnosis, management, and the importance of a multidisciplinary approach due to the lack of consensus on treatment.                                                                                                               | 2016 | Claire Dougan, Robyn Phillips, Ian Harley, et al.                                   | TOG                                                                         |
| Management of Bladder Pain Syndrome                                                                                   | This guideline provides evidence-based information for clinicians on the symptoms and treatment options for bladder pain syndrome (BPS) in women, highlighting the current uncertainties surrounding this condition.                                                                                                                                          | 2016 | Tirlapur SA, Birch JV, Carberry CL, et al.                                          | BJOG                                                                        |
| Making the best use of clinical datasets: with examples from urogynaecology                                           | This article explores the principles of data use, law, and ethics in clinical datasets, focusing on the importance of good data structure and analysis, with examples from urogynaecology.                                                                                                                                                                    | 2022 | Fiona Bach, Philip Toozs-Hobson, Jeremy Purnell                                     | TOG                                                                         |
| Accessory cavitated uterine malformations (ACUMs): an unfamiliar cause of dysmenorrhoea                               | The article reviews accessory cavitated uterine malformations (ACUMs), a rare Mullerian anomaly, as a cause of severe dysmenorrhoea and pelvic pain, discussing their diagnosis, treatment options, and the need for further research.                                                                                                                        | 2022 | Thulasi Setty, Joel Naftalin, Davor Jurkovic                                        | TOG                                                                         |
| Preterm labour and birth                                                                                              | This guideline covers the care of women with a singleton pregnancy at increased risk of, or with symptoms and signs of, preterm labour (before 37 weeks), and women with a singleton pregnancy having a planned preterm birth, aiming to reduce the risks of preterm birth for the baby and describing treatments to prevent or delay early labour and birth. | 2015 | –                                                                                   | NICE                                                                        |
| Heavy menstrual bleeding: assessment and management                                                                   | This guideline covers assessing and managing heavy menstrual bleeding, aiming to help healthcare professionals investigate the cause of heavy periods affecting a woman's quality of life and offer appropriate treatments.                                                                                                                                   | 2018 | –                                                                                   | NICE                                                                        |
| Pelvic exenteration for recurrent gynaecological cancer after radiotherapy                                            | The article discusses the challenges and considerations of pelvic exenteration for recurrent gynaecological cancers post-radiotherapy, emphasizing the importance of a multidisciplinary approach and the need for complete histological clearance for long-term survival.                                                                                    | 2017 | Desiree F Kolumainen, Desmond PJ Barton                                             | TOG                                                                         |

Continued on next page

Table 1 – continued from previous page

| Title                                                                                                                                                                                                                       | Synopsis                                                                                                                                                                                                                                                                        | Year | Authors                                                  | Publisher                                    |
|-----------------------------------------------------------------------------------------------------------------------------------------------------------------------------------------------------------------------------|---------------------------------------------------------------------------------------------------------------------------------------------------------------------------------------------------------------------------------------------------------------------------------|------|----------------------------------------------------------|----------------------------------------------|
| Effect of obesity on assisted reproductive treatment outcomes and its management: a literature review                                                                                                                       | This article reviews the impact of obesity on assisted reproductive treatment outcomes, exploring clinical outcomes, potential interventions, and ethical considerations.                                                                                                       | 2017 | Mohammed Khairy, Madhurima Rajkhowa                      | TOG                                          |
| Perinatal Management of Pregnant Women at the Threshold of Infant Viability (The Obstetric Perspective)                                                                                                                     | This paper discusses the medical and ethical challenges of managing pregnancies at the threshold of viability, focusing on optimizing perinatal care to improve survival and reduce morbidity in extremely preterm infants.                                                     | 2014 | Dr A Soe, Dr ALM David, Mr AD Roberts, et al.            | RCOG                                         |
| Valvular heart disease in pregnancy                                                                                                                                                                                         | This article discusses the challenges and management of valvular heart disease in pregnant women, emphasizing the importance of pre-conception counselling and multidisciplinary care.                                                                                          | 2023 | Paul Timmons, Gemma Partridge, Alastair McKelvey, et al. | TOG                                          |
| Management of cases relating to pregnancy, menopause, contraception and hysterectomy                                                                                                                                        | This guidance provides updated management protocols for pregnancy, menopause, contraception, and hysterectomy, focusing on cervical screening, colposcopy, and the use of contraceptives and hormone replacement therapy.                                                       | 2024 | –                                                        | NHS England                                  |
| Inflammatory bowel disease in pregnancy                                                                                                                                                                                     | This article provides an overview of inflammatory bowel disease (IBD) during pregnancy, discussing its impact on pregnancy, management strategies, and the safety of medications used to treat IBD in pregnant women.                                                           | 2016 | Dipanwita Kapoor, Kathy Teahon, Suzanne VF Wallace       | TOG                                          |
| Routes to parenthood for women with Turner syndrome                                                                                                                                                                         | This article discusses the reproductive challenges and options for women with Turner syndrome, including natural conception, assisted reproductive techniques, and ethical considerations.                                                                                      | 2019 | Mariano Mascarenhas, James Oliver, Harish M Bhandari     | TOG                                          |
| The management of haemoglobinopathies in pregnancy and childbirth                                                                                                                                                           | This article discusses the management of haemoglobinopathies, such as sickle cell disease and thalassaemias, during pregnancy and childbirth, emphasizing the importance of a multidisciplinary team approach for optimal maternal and fetal outcomes.                          | 2022 | Lucy A Jackson, Quentin A Hill, Etienne Ciantar          | TOG                                          |
| Sentinel Consensus Document for Vulval, Endometrial and Cervical Cancer BGCS January 2019                                                                                                                                   | The document discusses the consensus reached by the BGCS and UK gynaecological oncological community on the use of the sentinel lymph node technique in vulval, cervical, and endometrial cancer, including its applicability, safety, and implementation in UK cancer centres. | 2019 | Christina Fotopoulou, Thomas Ind, Peter Baldwin, et al.  | British Gynaecological Cancer Society (BGCS) |
| Joint British Association for Sexual Health and HIV and Royal College of Obstetricians and Gynaecologists national UK guideline for the management of herpes simplex virus (HSV) in pregnancy and the neonate (2024 update) | This updated national UK guideline provides recommendations for managing genital herpes simplex virus (HSV) in pregnant individuals and neonates, covering first episode and recurrent HSV, co-infection with HIV, and prevention of postnatal transmission.                    | 2024 | Emily Clarke, Raj Patel, Dyan Dickins, et al.            | International Journal of STD & AIDS          |
| Endometriosis                                                                                                                                                                                                               | The publication provides quality standards for the diagnosis and management of endometriosis, including guidelines for examinations, referrals, and treatment pathways.                                                                                                         | 2018 | –                                                        | NICE                                         |

Continued on next page

Table 1 – continued from previous page

| Title                                                                                                                                   | Synopsis                                                                                                                                                                                                                                          | Year | Authors                                                       | Publisher |
|-----------------------------------------------------------------------------------------------------------------------------------------|---------------------------------------------------------------------------------------------------------------------------------------------------------------------------------------------------------------------------------------------------|------|---------------------------------------------------------------|-----------|
| Impact of the intrauterine environment on future reproductive and metabolic health                                                      | The article explores how suboptimal intrauterine environments influence long-term reproductive and metabolic health outcomes, emphasizing the importance of maternal health and preconception care.                                               | 2022 | Suzanna Dunkerton, Catherine Aiken                            | TOG       |
| Placenta Praevia and Placenta Accreta: Diagnosis and Management                                                                         | This guideline provides an evidence-based approach to the diagnosis and management of pregnancies complicated by placenta praevia and placenta accreta, highlighting risk factors, diagnostic modalities, and management strategies.              | 2018 | ERM Jauniaux, Z Alfirevic, AG Bhide, et al.                   | RCOG      |
| Prenatal diagnosis in the modern era                                                                                                    | The article explores advancements in prenatal diagnosis, including noninvasive prenatal testing (NIPT), molecular genetic testing, and the integration of MRI with ultrasound, to enhance personalized antenatal care.                            | 2016 | Caroline E Fox, Mark D Kilby                                  | TOG       |
| A review of stroke in pregnancy: incidence, investigations and management                                                               | This article provides a comprehensive review on the clinical assessment, investigations, and treatment options for women presenting with stroke in pregnancy.                                                                                     | 2020 | Azriny S Khalid, Adriana Hadbavna, David Williams, et al.     | TOG       |
| Options for acquiring motherhood in absolute uterine factor infertility; adoption, surrogacy and uterine transplantation                | This review explores the options available for women with absolute uterine factor infertility (AUFU) to acquire motherhood, discussing the advantages and disadvantages of adoption, surrogacy, and uterine transplantation.                      | 2021 | Benjamin P Jones, Niccole Ranaei-Zamani, Saaliha Vali, et al. | TOG       |
| Prenatal Management of Pregnancies at Risk of Fetal Neonatal Alloimmune Thrombocytopenia (FNAIT)                                        | This paper discusses the latest evidence and treatment options for managing pregnancies at risk of Fetal Neonatal Alloimmune Thrombocytopenia (FNAIT), including the role of screening, immunoglobulin therapy, and potential future prophylaxis. | 2019 | F Regan, CC Lees, B Jones, et al.                             | RCOG      |
| Local Endometrial Trauma (Endometrial Scratch): A Treatment Strategy to Improve Implantation Rates Birth After Previous Caesarean Birth | This paper explores the potential benefits of local endometrial trauma, or 'endometrial scratch', as a strategy to improve implantation rates in assisted conception treatments, particularly for women with recurrent implantation failure.      | 2016 | Dr CJ Coughlan, Dr C Harrity, Professor SM Laird, et al.      | RCOG      |
| Trauma and pregnancy                                                                                                                    | This guideline provides evidence-based recommendations for antenatal and intrapartum care of women with previous caesarean delivery, focusing on options for vaginal birth after caesarean (VBAC) and elective repeat caesarean section (ERCS).   | 2015 | -                                                             | RCOG      |
| Diagnosing adnexal tumours before surgery: a critical appraisal of recent evidence                                                      | This article explores the impact of trauma on pregnant women, detailing the maternal and fetal complications, management strategies, and the importance of prioritizing the mother's health in trauma situations.                                 | 2021 | James Tibbott, Matteo Di Carlofelice, Rashmi Menon, et al.    | TOG       |
| Smoking in pregnancy: pathophysiology of harm and current evidence for monitoring and cessation                                         | The article critically appraises recent evidence on preoperative classification and diagnosis of ovarian and tubal neoplasms, discussing updated strategies and guidelines for optimal patient management.                                        | 2015 | Jeroen Kaijser, Kirsten Van Hoorde, Ben Van Calster, et al.   | TOG       |
|                                                                                                                                         | The article discusses the risks of smoking during pregnancy, the pathophysiology of harm caused by smoking, and evaluates current evidence for monitoring and cessation methods.                                                                  | 2019 | Brendan P McDonnell, Carmen Regan                             | TOG       |

Continued on next page

Table 1 – continued from previous page

| Title                                                                                                               | Synopsis                                                                                                                                                                                                                                                                                      | Year | Authors                                                       | Publisher |
|---------------------------------------------------------------------------------------------------------------------|-----------------------------------------------------------------------------------------------------------------------------------------------------------------------------------------------------------------------------------------------------------------------------------------------|------|---------------------------------------------------------------|-----------|
| Vasa Praevia: Diagnosis and Management                                                                              | This guideline provides an evidence-based approach to the diagnosis and management of pregnancies complicated by vasa praevia.                                                                                                                                                                | 2018 | ERM Jauniaux, Z Alfirevic, AG Bhide, et al.                   | RCOG      |
| Intrapartum care for women with existing medical conditions or obstetric complications and their babies             | This guideline covers care during labour and birth for women who need extra support due to medical conditions or complications in their current or previous pregnancy, as well as women who have had no antenatal care, aiming to improve experiences and outcomes for them and their babies. | 2019 | –                                                             | NICE      |
| Perinatal management of extreme preterm birth before 27 weeks of gestation: a framework for practice                | This framework provides guidance for the management of extremely preterm births before 27 weeks of gestation, emphasizing individualized care, parental involvement, and updated clinical practices to improve outcomes.                                                                      | 2020 | Helen Mactier, Sarah Elizabeth Bates, Tracey Johnston, et al. | BMJ       |
| Management of Beta Thalassaemia in Pregnancy                                                                        | This guideline provides evidence-based guidance on managing women with beta thalassaemia major and intermedia during pregnancy, covering preconceptual, antenatal, intrapartum, and postnatal care.                                                                                           | 2014 | Miss AAA Kyei-Mensah, Mr B Davis, Dr M Gupta, et al.          | RCOG      |
| Comprehensive review and update of cytomegalovirus infection in pregnancy                                           | This article provides a detailed review of cytomegalovirus (CMV) infection in pregnancy, discussing its prevalence, diagnosis, implications, and management options.                                                                                                                          | 2016 | Osric Navti, Brenna L Hughes, Julian W Tang, et al.           | TOG       |
| Vascular injury during laparoscopic gynaecological surgery: a methodological approach for prevention and management | This article discusses the prevention and management of vascular injuries during laparoscopic gynaecological surgery, highlighting risk factors, techniques, and protocols to minimize morbidity and mortality.                                                                               | 2020 | Gemma Brierley, Ilyas Arshad, Fevzi Shakir, et al.            | TOG       |
| Sports gynaecology                                                                                                  | The article explores the health implications of long-term intense exercise on elite sportswomen, focusing on conditions like Relative Energy Deficiency in Sport (RED-S) and its impact on menstrual abnormalities, subfertility, and urinary incontinence.                                   | 2019 | Benjamin P Jones, Ariadne L'Heveder, Srdjan Saso, et al.      | TOG       |
| Endometrial cancer and obesity                                                                                      | This article explores the strong association between obesity and endometrial cancer, discussing mechanisms, prevention, diagnosis, and treatment challenges in obese women.                                                                                                                   | 2019 | Sarah J Kitson, Emma J Crosbie                                | TOG       |
| Shared decision making                                                                                              | This guideline covers how to make shared decision making part of everyday care in all healthcare settings, promoting collaboration between healthcare professionals and service users to make informed decisions about treatment and care.                                                    | 2021 | –                                                             | NICE      |
| Laparoscopic myomectomy: a review of alternatives, techniques and controversies                                     | This article reviews the techniques, alternatives, and controversies surrounding laparoscopic myomectomy, focusing on surgical challenges, patient selection, and the risks associated with morcellation.                                                                                     | 2018 | Alison Bryant-Smith, Tom Holland                              | TOG       |
| Oophorectomy or ovarian conservation at the time of hysterectomy for benign disease                                 | The article discusses the decision-making process and implications of performing oophorectomy versus ovarian conservation during hysterectomy for benign conditions, highlighting the risks and benefits associated with each approach.                                                       | 2022 | Victoria Asfour, Adam D Jakes, Jess McMicking, et al.         | TOG       |
| Pelvic floor functional bowel disorders in gynaecology                                                              | This article discusses the common pelvic floor bowel disorders seen in gynaecology clinics, their investigations, and treatment, emphasizing a multidisciplinary approach to management.                                                                                                      | 2020 | Marika Britton, Sushil Maslekar, Fiona Marsh                  | TOG       |

Continued on next page

Table 1 – continued from previous page

| Title                                                                                                                     | Synopsis                                                                                                                                                                                                                                                                                         | Year | Authors                                                         | Publisher                       |
|---------------------------------------------------------------------------------------------------------------------------|--------------------------------------------------------------------------------------------------------------------------------------------------------------------------------------------------------------------------------------------------------------------------------------------------|------|-----------------------------------------------------------------|---------------------------------|
| The Management of Ovarian Hyperstimulation Syndrome                                                                       | This guideline provides evidence-based advice for diagnosing and managing ovarian hyperstimulation syndrome (OHSS), a complication of fertility treatment, focusing on early recognition and prompt assessment and treatment.                                                                    | 2016 | –                                                               | RCOG                            |
| Unscheduled bleeding with hormone replacement therapy                                                                     | This article discusses the challenges and management of unscheduled bleeding in women undergoing hormone replacement therapy (HRT), emphasizing the need for appropriate investigation and treatment to exclude endometrial pathology and maintain patient compliance.                           | 2019 | Fulva Gajjar Dave, Tolu Adedipe, Stewart Disu, et al.           | TOG                             |
| Making Safe Abortion                                                                                                      | The publication outlines best practices in post-abortion care and medically indicated abortions, aiming to reduce maternal mortality and morbidity by providing safe and accessible abortion services.                                                                                           | 2022 | Anna Glasier, David Baird, Paul Blumenthal, et al.              | RCOG                            |
| Clamping of the Umbilical Cord and Placental Transfusion                                                                  | This paper reviews the physiology of placental transfusion and evaluates the evidence related to the timing of umbilical cord clamping.                                                                                                                                                          | 2015 | Professor LMM Duley, Professor JO Drife, Dr A Soe, et al.       | RCOG                            |
| Perinatal mental health: how to ask and how to help                                                                       | The article discusses strategies for obstetricians to effectively address and manage perinatal mental health issues, emphasizing the importance of open communication and risk assessment.                                                                                                       | 2017 | Gabrielle A Bambridge, Elizabeth J Shaw, Melania Ishak, et al.  | TOG                             |
| Bacterial Sepsis following Pregnancy                                                                                      | This guideline provides guidance on the management of sepsis in the puerperium, focusing on the recognition, investigation, and management strategies for bacterial sepsis post-pregnancy.                                                                                                       | 2012 | –                                                               | RCOG                            |
| Analgesia for labour: an evidence-based insight for the obstetrician                                                      | The article provides an overview of analgesic options for labour, discussing both pharmacological and non-pharmacological methods, with a focus on evidence-based practices and the importance of caregiver attitude in pain management.                                                         | 2015 | Djavid I Alleemudder, Yemi Kuponiyi, Charlotte Kuponiyi, et al. | TOG                             |
| Clinical reflective practice                                                                                              | The article discusses the importance of reflective practice in medical education and clinical development, highlighting its role in enhancing knowledge, understanding, and professional development.                                                                                            | 2020 | Ruth Roberts, Bid Kumar                                         | TOG                             |
| Metformin Therapy for the Management of Infertility in Women with Polycystic Ovary Syndrome                               | This paper discusses the use of metformin therapy for managing infertility in women with polycystic ovary syndrome, evaluating its effects on reproductive outcomes and associated metabolic parameters.                                                                                         | 2017 | Dr LC Morley, Dr TMH Tang, Professor AH Balen                   | RCOG                            |
| Hyperlipidaemia and severe hypertriglyceridaemia in pregnancy                                                             | The article discusses the physiological changes in lipid levels during pregnancy, the complications associated with hypercholesterolaemia and severe hypertriglyceridaemia, and management strategies for these conditions.                                                                      | 2023 | Mohammed Bashir, Osric B Navti, Badreldeen Ahmed, et al.        | TOG                             |
| British HIV Association guidelines for the management of HIV in pregnancy and postpartum 2018 (2020 third interim update) | These guidelines provide best clinical practice guidance for the treatment and management of women living with HIV in the UK during pregnancy and postpartum, including the use of antiretroviral therapy to prevent vertical transmission and recommendations for specific patient populations. | 2020 | Dr Yvonne Gilleece, Dr Shema Tariq, Ms Funmi Awosusi, et al.    | British HIV Association (BHIVA) |
| Bacterial Sepsis in Pregnancy                                                                                             | This guideline addresses the recognition and management of serious bacterial illness in pregnancy, focusing on antenatal and intrapartum periods, and highlights the importance of early recognition and treatment to improve maternal outcomes.                                                 | 2012 | Dr D Pasupathy, Dr M Morgan, Dr FS Plaat, et al.                | RCOG                            |

Continued on next page

Table 1 – continued from previous page

| Title                                                                                                                                  | Synopsis                                                                                                                                                                                                                            | Year | Authors                                                                   | Publisher                            |
|----------------------------------------------------------------------------------------------------------------------------------------|-------------------------------------------------------------------------------------------------------------------------------------------------------------------------------------------------------------------------------------|------|---------------------------------------------------------------------------|--------------------------------------|
| Management of women with postmenopausal bleeding: evidence-based review                                                                | This article reviews modern management strategies for women with postmenopausal bleeding, focusing on evidence-based approaches to investigation and diagnosis.                                                                     | 2012 | Shagaf H Bakour, Anne Timmermans, Ben Willem Mol, et al.                  | TOG                                  |
| Life in the laparoscopic fast lane: evidence-based perioperative management and enhanced recovery in benign gynaecological laparoscopy | This article discusses evidence-based perioperative management and enhanced recovery protocols in benign gynaecological laparoscopy to improve patient outcomes and satisfaction.                                                   | 2021 | Alison Bryant-Smith, Sawsan As-Sanie, Jillian Lloyd, et al.               | TOG                                  |
| Investigation and management of postcoital bleeding                                                                                    | This article reviews the causes, assessment, and management of postcoital bleeding, emphasizing the importance of excluding cervical cancer and providing a framework for clinical evaluation.                                      | 2022 | Gemma L Owens, Nick J Wood, Pierre Martin-Hirsch                          | TOG                                  |
| Peripartum hyponatraemia: an overview of physiology, prevention and management                                                         | This article discusses the physiology, prevention, and management of peripartum hyponatraemia, a common but underreported condition that can significantly impact maternal and neonatal outcomes.                                   | 2022 | Eleftheria Demertzidou, Rabia Zill-E-Huma, Mona Modi                      | TOG                                  |
| The management of pregnant women with epilepsy: a multidisciplinary collaborative approach to care                                     | This article discusses the management of epilepsy in pregnant women, emphasizing the need for a multidisciplinary approach to improve outcomes and reduce risks associated with anti-epileptic drugs and seizures during pregnancy. | 2017 | Meena Bhatia, Jane E Adcock, Lucy Mackillop                               | TOG                                  |
| Chickenpox in Pregnancy                                                                                                                | This guideline addresses the prevention and management of varicella (chickenpox) infection in pregnant women, including vaccination, post-exposure prophylaxis, and the risks to both mother and fetus.                             | 2024 | –                                                                         | RCOG                                 |
| Placental histopathological abnormalities and poor perinatal outcomes                                                                  | This article examines the correlation between placental histology and adverse perinatal outcomes, highlighting the importance of placental examination in understanding and managing pregnancy complications.                       | 2019 | Lakshmi Thirumalaikumar, Kalaivani Ramalingam, Tamas Marton               | TOG                                  |
| 2018 ESC Guidelines for the management of cardiovascular diseases during pregnancy                                                     | The guidelines provide comprehensive recommendations for managing cardiovascular diseases during pregnancy, emphasizing risk assessment, treatment options, and the importance of a multidisciplinary approach.                     | 2018 | Vera Regitz-Zagrosek, Jolien W. Roos-Hesselink, Johann Bauersachs, et al. | European Society of Cardiology (ESC) |
| Management of uterine prolapse: is hysterectomy necessary?                                                                             | The article explores the management options for uterine prolapse, debating the necessity of hysterectomy versus uterine preservation surgery.                                                                                       | 2016 | Helen Jefferis, Simon Robert Jackson, Natalia Price                       | TOG                                  |
| Obstetric Neurological Injuries                                                                                                        | The article discusses the uncommon but potentially serious neurological injuries following childbirth, emphasizing their causes, diagnosis, and management, with a focus on distinguishing them from anaesthesia-related injuries.  | 2020 | Robert LC Harper, Seumas D Eckford, Helen Williams, et al.                | TOG                                  |
| Management and referral guidelines for colposcopy                                                                                      | This document provides updated guidelines for the management and referral processes in colposcopy, focusing on standards for cervical screening, hrHPV testing, and follow-up procedures.                                           | 2024 | –                                                                         | NHS England                          |
| Catheter use in gynaecological practice                                                                                                | The article discusses the indications, types, and complications of catheter use in gynaecological practice, emphasizing the need for proper training and patient education.                                                         | 2014 | Nosheen Aslam, Paul A Moran                                               | TOG                                  |

Continued on next page

Table 1 – continued from previous page

| Title                                                                                                        | Synopsis                                                                                                                                                                                                                                                                                                         | Year | Authors                                                                                                            | Publisher |
|--------------------------------------------------------------------------------------------------------------|------------------------------------------------------------------------------------------------------------------------------------------------------------------------------------------------------------------------------------------------------------------------------------------------------------------|------|--------------------------------------------------------------------------------------------------------------------|-----------|
| The use and abuse of oxytocin                                                                                | The article discusses the historical and current use of oxytocin in labour management, highlighting its benefits and risks, and emphasizes the need for better education and training to prevent misuse.                                                                                                         | 2015 | Karl SJ Oláh, Philip J Steer                                                                                       | TOG       |
| Preventing Entry-Related Gynaecological Laparoscopic Injuries                                                | This guideline aims to highlight strategies to reduce complications during laparoscopic surgery, focusing on the entry-related injuries that occur during the blind insertion of needles, trocars, and cannulae.                                                                                                 | –    | Professor CJG Sutton FRCOG, Guildford, and Mr K Philips FRCOG, et al.                                              | RCOG      |
| The management of endometrial polyps in the 21st century                                                     | This article reviews the diagnosis and management of endometrial polyps, highlighting the superiority of hysteroscopic removal over blind avulsion and discussing the implications for fertility and malignancy risk.                                                                                            | 2012 | John Jude Annan, Joseph Aquilina, Elizabeth Ball                                                                   | TOG       |
| Consent Advice No. 12: Caesarean Section for Placenta Praevia                                                | This guidance provides additional advice for clinicians on obtaining consent for caesarean section in cases of placenta praevia, highlighting specific risks and considerations.                                                                                                                                 | 2010 | Mr E P Morris FRCOG with the support of the Consent Group of the Royal College of Obstetricians and Gynaecologists | RCOG      |
| Prevention and Management of Postpartum Haemorrhage                                                          | This guideline provides comprehensive recommendations for the prevention and management of postpartum haemorrhage, including risk factors, treatment protocols, and the role of various medical interventions.                                                                                                   | 2016 | Mavrides E, Allard S, Chandraran E, et al.                                                                         | RCOG      |
| Premenstrual disorders including premenstrual syndrome and premenstrual dysphoric disorder                   | This article explores the spectrum of premenstrual disorders, focusing on the pathophysiology, diagnosis, and treatment options for conditions like premenstrual syndrome (PMS) and premenstrual dysphoric disorder (PMDD), highlighting their impact on women's quality of life.                                | 2023 | Nidhi Goswami, Kalpana Upadhyay, Paula Briggs, et al.                                                              | TOG       |
| Neonatal infection: antibiotics for prevention and treatment                                                 | This guideline covers preventing bacterial infection in healthy babies up to 28 days old, treating pregnant women whose unborn baby is at risk of infection, and caring for babies with suspected or confirmed bacterial infection, aiming to reduce delays in treatment and prevent unnecessary antibiotic use. | 2021 | –                                                                                                                  | NICE      |
| Menopause: identification and management                                                                     | This guideline covers identifying and managing menopause, including in people with premature ovarian insufficiency, aiming to improve the consistency of support and information provided to people experiencing menopause.                                                                                      | 2024 | –                                                                                                                  | NICE      |
| Advanced abdominal pregnancy: challenges, update and review of current management                            | This article reviews the challenges, updates, and current management strategies for advanced abdominal pregnancy, a rare and potentially life-threatening condition.                                                                                                                                             | 2022 | Anna McDougall, Amelie Morin, Tatiana Kuzmich, et al.                                                              | TOG       |
| Pelvic and vaginal packing for intractable venous obstetric haemorrhage: practical tips for the obstetrician | This article provides practical guidance and tips for obstetricians on performing pelvic and vaginal packing to manage intractable venous obstetric haemorrhage.                                                                                                                                                 | 2014 | Wai Yoong, Viswa Sivashanmugarajan, Morgan McMonagle, et al.                                                       | TOG       |
| Giving effective feedback in medical education                                                               | This article discusses the importance of effective feedback in medical education, outlining models and principles for providing feedback to enhance learning and development in trainees.                                                                                                                        | 2017 | Najum S Qureshi                                                                                                    | TOG       |
| Blood Transfusion in Obstetrics                                                                              | This guideline provides updated recommendations on the appropriate use of blood products in obstetrics to minimize risks and manage obstetric haemorrhage effectively.                                                                                                                                           | 2015 | –                                                                                                                  | RCOG      |

Continued on next page

Table 1 – continued from previous page

| Title                                                                                        | Synopsis                                                                                                                                                                                                                                                   | Year | Authors                                                                                       | Publisher |
|----------------------------------------------------------------------------------------------|------------------------------------------------------------------------------------------------------------------------------------------------------------------------------------------------------------------------------------------------------------|------|-----------------------------------------------------------------------------------------------|-----------|
| Reproductive Outcomes after Local Treatment for Preinvasive Cervical Disease                 | This paper reviews the impact of local cervical treatment for preinvasive cervical disease on reproductive outcomes, including fertility, early pregnancy, and obstetric outcomes, with a focus on UK practices.                                           | 2016 | Dr M Kyrgiou MRCOG, Dr PL Martin-Hirsch FRCOG, Professor EA Paraskevaidis, et al.             | RCOG      |
| ST analysis for intrapartum fetal monitoring                                                 | The article discusses the use of ST analysis (STAN) as an adjunct to cardiotocography (CTG) for intrapartum fetal monitoring, highlighting its potential benefits and limitations.                                                                         | 2015 | Adalina Sacco, Javaid Muglu, Ramesan Navaratnarajah, et al.                                   | TOG       |
| A review of contraceptive methods for women with cardiac disease                             | The article discusses the importance of effective contraception in women with cardiac disease, providing information for healthcare professionals to counsel these women on contraceptive options.                                                         | 2018 | Adam D Jakes, Felicity Coad, Catherine Nelson-Piercy                                          | TOG       |
| Obtaining Valid Consent to Participate in Perinatal Research Where Consent is Time Critical  | This guidance provides a framework for researchers on obtaining valid consent for perinatal research when time is critical, focusing on the timing and detail of study information provision and consent during labour or the immediate postpartum period. | 2016 | Dr S Kenyon PhD, MA, RM, et al.                                                               | RCOG      |
| Jaundice in newborn babies under 28 days                                                     | This guideline covers diagnosing and treating jaundice in newborn babies, aiming to detect or prevent harmful levels of bilirubin.                                                                                                                         | 2010 | –                                                                                             | NICE      |
| The use of urethral bulking agents in the treatment of stress urinary incontinence           | This article discusses the use of urethral bulking agents as a treatment for stress urinary incontinence, examining their efficacy, complications, and the impact of the UK pause on mesh use.                                                             | 2020 | Shaun McGowan, Patrick Campbell, Lucia Dolan                                                  | TOG       |
| Female sexual dysfunction                                                                    | This article provides an update on female sexual dysfunction terminology, explores various gynaecological problems and their effects on sexual function, and assesses the effectiveness of therapeutic modalities.                                         | 2022 | Victoria Kershaw, Swati Jha                                                                   | TOG       |
| Management of borderline ovarian tumours                                                     | The article discusses the management strategies for borderline ovarian tumours, emphasizing surgical staging, fertility-sparing options, and the role of multidisciplinary teams.                                                                          | 2012 | Pallavi Bagade, Richard Edmondson, Anitha Nayar                                               | TOG       |
| Management of Premenstrual Syndrome                                                          | This guideline reviews the diagnosis, classification, and management of premenstrual syndrome (PMS), examining both pharmacological and non-pharmacological treatments.                                                                                    | 2017 | Green LJ, O'Brien PMS, Panay N, et al.                                                        | RCOG      |
| Planned Caesarean Birth Pain Relief and Informed Decision Making for Outpatient Hysteroscopy | This guidance aims to optimize women's experience and clinical outcomes in outpatient hysteroscopy by providing clear information and advocating for informed decision-making regarding pain relief and procedural options.                                | 2023 | Professor TJ Clark FRCOG, Mr E Morris FRCOG, Mr J Lord FRCOG, et al.                          | RCOG      |
| Medicolegal update on consent: 'The Montgomery Ruling'                                       | The article discusses the impact of the Montgomery ruling on informed consent in medical practice, highlighting the shift from a paternalistic approach to a patient-centered one, particularly in obstetrics and gynaecology.                             | 2015 | Elaine Cheung, Gemma Goodyear, Wai Yoong                                                      | –         |
| The Role of Emergency and Elective Interventional Radiology in Postpartum Haemorrhage        | This guidance urges obstetric units to consider interventional radiology as a tool in preventing and managing postpartum haemorrhage, potentially reducing the need for blood transfusion and hysterectomy.                                                | 2007 | Professor S Arulkumaran FRCOG, Professor JJ Walker FRCOG, Professor AF Watkinson FRCR, et al. | RCOG      |
| Raised CA125 – what we actually know...                                                      | The article explores the role of CA125 in diagnosing ovarian cancer, its limitations, and its implications in clinical practice.                                                                                                                           | 2020 | Tamara Howe, Nava Sokolovsky, Ahmad Sayasneh, et al.                                          | TOG       |

Continued on next page

Table 1 – continued from previous page

| Title                                                                                                             | Synopsis                                                                                                                                                                                                                                                                                                                                 | Year | Authors                                                                                                         | Publisher |
|-------------------------------------------------------------------------------------------------------------------|------------------------------------------------------------------------------------------------------------------------------------------------------------------------------------------------------------------------------------------------------------------------------------------------------------------------------------------|------|-----------------------------------------------------------------------------------------------------------------|-----------|
| Risk-Reducing Salpingo-Oophorectomy and the Use of Hormone Replacement Therapy Below the Age of Natural Menopause | This paper discusses the use of hormone replacement therapy (HRT) after the removal of fallopian tubes and ovaries to prevent ovarian cancer in premenopausal high-risk women, addressing the implications of early menopause and the need for guidance on post-surgery care.                                                            | 2022 | R Manchanda, F Gaba, V Talaulikar, et al.                                                                       | RCOG      |
| Headaches in pregnancy                                                                                            | The article reviews the management of common causes of headaches in pregnancy, emphasizing the importance of distinguishing between benign and potentially life-threatening conditions.                                                                                                                                                  | 2014 | Kirsty Revell, Paul Morrish                                                                                     | TOG       |
| Human papillomavirus-independent cervical cancer and its precursor lesions                                        | The article discusses the increasing recognition of HPV-independent cervical cancers, particularly adenocarcinomas, and highlights the need for awareness among clinicians due to their worse prognosis compared to HPV-associated adenocarcinomas.                                                                                      | 2023 | Ieera Madan Aggarwal, Yen Ching Yeo, Zheng Yuan Ng                                                              | TOG       |
| Uterine Transplantation                                                                                           | This paper explores uterine transplantation as a potential treatment for women with absolute uterine factor infertility, discussing its risks, benefits, and the framework for establishing a sustainable program.                                                                                                                       | 2021 | BP Jones, S Saso, J Yazbek, et al.                                                                              | RCOG      |
| Laparoscopic Management of Tubal Ectopic Pregnancy                                                                | This guidance provides advice for clinicians on obtaining consent for laparoscopic salpingectomy or salpingotomy in cases of ectopic pregnancy, ensuring women receive consistent and adequate information.                                                                                                                              | 2010 | Mr M Read FRCOG, with the support of the Consent Group of the Royal College of Obstetricians and Gynaecologists | RCOG      |
| Antenatal venous thromboembolism                                                                                  | The article discusses the challenges and management strategies for diagnosing and treating venous thromboembolism (VTE) during pregnancy, emphasizing the role of low-molecular-weight heparin and the importance of multidisciplinary care.                                                                                             | 2021 | David A Crosby, Ann McHugh, Kevin Ryan, et al.                                                                  | TOG       |
| Caesarean scar ectopic pregnancy: diagnostic challenges and management options                                    | The article discusses the increasing incidence of caesarean scar pregnancy (CSP), its diagnostic challenges, and various management options, emphasizing the importance of prompt diagnosis and individualized treatment to reduce morbidity.                                                                                            | 2017 | Pradeep M Jayaram, Gbemisola O Okunoye, Justin Konje                                                            | TOG       |
| Preterm labour and birth                                                                                          | This guideline covers the care of women with a singleton pregnancy at increased risk of, or with symptoms and signs of, preterm labour, aiming to reduce risks for the baby and describes treatments to prevent or delay early labour and birth.                                                                                         | 2015 | –                                                                                                               | NICE      |
| Preterm labour and birth                                                                                          | This guideline covers the care of women with a singleton pregnancy at increased risk of, or with symptoms and signs of, preterm labour (before 37 weeks), and women with a singleton pregnancy having a planned preterm birth, aiming to reduce risks for the baby and describing treatments to prevent or delay early labour and birth. | 2015 | –                                                                                                               | NICE      |
| Enhanced recovery in gynaecology                                                                                  | Enhanced recovery pathways improve the quality and experience of care for patients undergoing elective gynaecology surgery by enabling quicker recovery and reducing hospital stay.                                                                                                                                                      | 2013 | Emma Torbe, Robin Crawford, Andy Nordin, et al.                                                                 | TOG       |
| Postpartum contraception                                                                                          | The article discusses the importance of initiating contraception in the postpartum period to prevent unintended pregnancies and short inter-pregnancy intervals, highlighting the role of maternity services in providing contraceptive options immediately after childbirth.                                                            | 2018 | Michelle Cooper, Sharon Cameron                                                                                 | TOG       |

Continued on next page

Table 1 – continued from previous page

| Title                                                                                                    | Synopsis                                                                                                                                                                                                                                                                                                                                              | Year | Authors                                                                 | Publisher                                    |
|----------------------------------------------------------------------------------------------------------|-------------------------------------------------------------------------------------------------------------------------------------------------------------------------------------------------------------------------------------------------------------------------------------------------------------------------------------------------------|------|-------------------------------------------------------------------------|----------------------------------------------|
| A focus on progestogens in hormone replacement therapy                                                   | The article discusses the role of progestogens in hormone replacement therapy, highlighting their benefits, side effects, and the importance of tailoring treatment to individual patients.                                                                                                                                                           | 2023 | Srirupa Ghosh, Rachel Imrie, James Goadsby, et al.                      | TOG                                          |
| Multifetal pregnancy reduction and selective termination                                                 | This article discusses the indications, technical considerations, outcomes, and ethical issues surrounding multifetal pregnancy reduction (MFPR) and selective termination (ST) in multifetal pregnancies.                                                                                                                                            | 2020 | Sridevi Beriwai, Lawrence Impey, Christos Ioannou                       | TOG                                          |
| British Gynaecological Cancer Society (BGCS) Uterine Cancer Guidelines: Recommendations for Practice     | This guideline provides evidence-based recommendations for the diagnosis and management of uterine cancer, covering all histological types.                                                                                                                                                                                                           | –    | Jo Morrison, Janos Balega, Lynn Buckley, et al.                         | British Gynaecological Cancer Society (BGCS) |
| Lynch syndrome for the gynaecologist                                                                     | This article discusses Lynch syndrome, an autosomal dominant condition associated with colorectal, endometrial, and ovarian cancer, emphasizing the importance of personalized counselling, testing strategies, and risk-reducing strategies for women with the syndrome.                                                                             | 2021 | Neil AJ Ryan, Raymond FT McMahon, Neal C Ramchander, et al.             | TOG                                          |
| Maternal, fetal, and neonatal outcomes associated with long-term use of corticosteroids during pregnancy | This article reviews the maternal, fetal, and neonatal effects of chronic corticosteroid use during pregnancy, discussing whether additional antenatal corticosteroids are necessary for preterm delivery.                                                                                                                                            | 2019 | Doua AlSaad, Stephen Lindow, Ben H Lee, et al.                          | TOG                                          |
| Roles and responsibilities of the consultant providing acute care in obstetrics and gynaecology          | This paper refines the roles and responsibilities of consultants in obstetrics and gynaecology, emphasizing leadership, team collaboration, and patient care standards.                                                                                                                                                                               | 2021 | Barber JS, Cunningham S, Mountfield J, et al.                           | RCOG                                         |
| Phenylketonuria in pregnancy                                                                             | The article discusses the management and implications of phenylketonuria (PKU) in pregnancy, emphasizing the importance of a multidisciplinary approach and dietary control to prevent fetal abnormalities.                                                                                                                                           | 2018 | Carol R Munyame, Nirmala Vaithilingam, Yusof Rahman, et al.             | TOG                                          |
| Surgical Management of Miscarriage and Removal of Persistent Placental or Fetal Remains                  | This guidance provides advice for health professionals on obtaining consent from women undergoing surgical management of miscarriage, ensuring consistent and adequate information is given for consent.                                                                                                                                              | 2018 | Dr DM Siassakos MRCOG, Dr JA Hamilton MRCOG, Dr SD Newell MRCOG, et al. | RCOG                                         |
| Management of common disorders in psychosexual medicine                                                  | This article outlines the management of psychosexual dysfunction in the gynaecology outpatient department, emphasizing the importance of psychosexual medicine training and the need for enhanced consultation skills to address common disorders such as sexual pain disorders, hypoactive sexual desire disorder, and persistent vaginal discharge. | 2015 | Fiona Cowan, Leila Frodsham                                             | TOG                                          |
| Diabetes insipidus in pregnancy                                                                          | The article discusses the types, diagnosis, and management of diabetes insipidus during pregnancy, highlighting the importance of early detection and multidisciplinary care to reduce morbidity and mortality for both mother and fetus.                                                                                                             | 2018 | James Quigley, Cliff Shelton, Basil Issa, et al.                        | TOG                                          |
| Umbilical Cord Prolapse                                                                                  | This guideline provides recommendations for the prevention, diagnosis, and management of umbilical cord prolapse in both hospital and community settings.                                                                                                                                                                                             | 2014 | –                                                                       | RCOG                                         |

Continued on next page

Table 1 – continued from previous page

| Title                                                                                                   | Synopsis                                                                                                                                                                                                                                                                     | Year | Authors                                                                     | Publisher |
|---------------------------------------------------------------------------------------------------------|------------------------------------------------------------------------------------------------------------------------------------------------------------------------------------------------------------------------------------------------------------------------------|------|-----------------------------------------------------------------------------|-----------|
| Acute colonic pseudo-obstruction after caesarean section: a review and recommended management algorithm | This article reviews the pathophysiology, presentation, diagnosis, and management of acute colonic pseudo-obstruction (ACPO) following caesarean section, providing an algorithm for optimal management aimed at obstetric clinicians and general surgeons.                  | 2019 | Alice E Hughes, Neil J Smart, Ian R Daniels                                 | TOG       |
| Shoulder Dystocia                                                                                       | This guideline reviews the current evidence regarding the prediction, prevention, and management of shoulder dystocia, providing guidance for skills training but not detailing practical manoeuvres.                                                                        | 2012 | Dr J Crofts MRCOG, Professor TJ Draycott MRCOG, Dr I Montague FRCOG, et al. | RCOG      |
| FIGO Ovarian Cancer Staging Effective Jan. 1, 2014                                                      | The article outlines the updated FIGO staging system for ovarian cancer, effective from January 1, 2014, highlighting changes in staging criteria and additional recommendations.                                                                                            | 2014 | –                                                                           | FIGO      |
| Syphilis in pregnancy: identifying and managing a historic problem on the rise                          | The article discusses the rising incidence of syphilis in pregnancy, its implications for maternal and fetal health, and the importance of timely diagnosis and treatment to prevent congenital syphilis.                                                                    | 2020 | Louise Dewick, Kanna Jayaprakasan, Sanaria Raouf                            | TOG       |
| A practical guide to appraisal and revalidation                                                         | The article provides guidance on the appraisal and revalidation process for obstetricians and gynaecologists, emphasizing the importance of supporting information and professional development.                                                                             | 2018 | Catharina Schram MH                                                         | TOG       |
| The clinical application of transperineal ultrasound in urogynaecology                                  | This article discusses the use of transperineal ultrasound as a tool for diagnosing and treating urogynaecological conditions, highlighting its application in assessing pelvic floor disorders, urinary incontinence, and birth trauma.                                     | 2022 | Francois Retief, Frances Paterson, Jakub Jagiellowicz, et al.               | TOG       |
| Preimplantation genetic diagnosis: an overview and recent advances                                      | This article discusses the development, indications, and ethical considerations of preimplantation genetic diagnosis (PGD), highlighting recent advances in genetic diagnosis methods and the process of in vitro fertilisation for PGD.                                     | 2016 | Jara Ben-Nagi, Paul Serhal, Sioban Sengupta, et al.                         | TOG       |
| Antenatal venous thromboembolism                                                                        | This article discusses the management of antenatal venous thromboembolism, including guidance on treatment and ultrasound follow-up.                                                                                                                                         | 2021 | Crosby DA, McHugh A, Ryan K, et al.                                         | TOG       |
| Female Genital Mutilation and its Management                                                            | This guideline provides evidence-based guidance on the management of women with female genital mutilation (FGM) and those at risk, covering clinical care before, during, and after pregnancy, as well as the legal and regulatory responsibilities of health professionals. | 2015 | –                                                                           | RCOG      |
| Surgical site infection in obstetrics and gynaecology: prevention and management                        | This article discusses the prevention and management of surgical site infections (SSIs) in obstetrics and gynaecology, highlighting risk factors, prevention strategies, and the role of antibiotics.                                                                        | 2021 | Emmanuel E Ekanem, Olubunmi Oniya, Hudah Saleh, et al.                      | TOG       |
| Acute kidney injury in pregnancy and the use of non-steroidal anti-inflammatory drugs                   | The article discusses the causes, diagnosis, and management of acute kidney injury (AKI) in pregnancy, with a focus on the risks associated with non-steroidal anti-inflammatory drugs (NSAIDs).                                                                             | 2016 | Kate S Wiles, Anita Banerjee                                                | TOG       |
| Management of Suspected Ovarian Masses in Premenopausal Women                                           | This guideline provides information to assist clinicians with the assessment and management of suspected ovarian masses in premenopausal women, focusing on when to manage within a benign gynaecological service and when to refer to a gynaecological oncological service. | 2011 | Mr PD Kaloo MRCOG, Mr KA Loudon FRCOG, Mr S Khazali MRCOG, et al.           | RCOG      |

Continued on next page

Table 1 – continued from previous page

| Title                                                                    | Synopsis                                                                                                                                                                                                                                                            | Year | Authors                                                                                                                         | Publisher                                                                                                                                              |
|--------------------------------------------------------------------------|---------------------------------------------------------------------------------------------------------------------------------------------------------------------------------------------------------------------------------------------------------------------|------|---------------------------------------------------------------------------------------------------------------------------------|--------------------------------------------------------------------------------------------------------------------------------------------------------|
| FIGO staging for carcinoma of the vulva: 2021 revision                   | The 2021 revision of FIGO staging for carcinoma of the vulva introduces a data-driven approach to simplify and improve prognostic accuracy, incorporating new definitions and cross-sectional imaging findings.                                                     | 2021 | Alexander B. Olawaiye, Joseph Cotler, Mauricio A. Cuello, et al.                                                                | International Journal of Gynecology & Obstetrics published by John Wiley & Sons Ltd on behalf of International Federation of Gynecology and Obstetrics |
| Care of late intrauterine fetal death and stillbirth                     | This guideline provides evidence-based recommendations for the care of parents and families experiencing late intrauterine fetal death (IUFD) after 24 weeks of pregnancy, focusing on options for induction of labour, communication, and post-mortem examination. | 2024 | Christy Burden, Abi Merriel, Danya Bakhbakhi, et al.                                                                            | RCOG                                                                                                                                                   |
| Iron deficiency and iron-deficiency anaemia in women's health            | This article reviews the aetiology, assessment, and management of iron deficiency and iron-deficiency anaemia in women's health, highlighting the importance of diagnosis and treatment to improve quality of life.                                                 | 2017 | Laura Percy, Diana Mansour                                                                                                      | TOG                                                                                                                                                    |
| Reproductive Implications and Management of Congenital Uterine Anomalies | This paper discusses congenital uterine anomalies, their reproductive implications, diagnostic methods, and management options, emphasizing the need for evidence-based recommendations for surgical treatment.                                                     | 2020 | MA Akhtar, SH Saravelos, TC Li, et al.                                                                                          | RCOG                                                                                                                                                   |
| Surgical smoke – what are the risks?                                     | The article reviews the sources, components, and effects of surgical smoke, highlighting the potential health risks and recommending protective measures for operating theatre staff.                                                                               | 2019 | Susan Addley, Declan Quinn                                                                                                      | TOG                                                                                                                                                    |
| Abdominal Hysterectomy for Benign Conditions                             | This guidance provides advice for clinicians on obtaining consent for women undergoing abdominal hysterectomy under general anaesthesia, ensuring consistent and adequate information is given for consent.                                                         | 2009 | Dr LC Edozien FRCOG, Manchester, with the support of the Consent Group of the Royal College of Obstetricians and Gynaecologists | RCOG                                                                                                                                                   |
| Amniocentesis and chorionic villus sampling                              | This guideline provides evidence-based standards for the provision and performance of amniocentesis and chorionic villus sampling (CVS) used for prenatal diagnosis.                                                                                                | 2021 | K Navaratnam, Z Alfrevic                                                                                                        | RCOG                                                                                                                                                   |
| Unexplained subfertility: diagnosis and management                       | This article discusses the diagnosis and management of unexplained subfertility, highlighting potential contributing factors and treatment options amidst ongoing debates in the field.                                                                             | 2016 | Anupa Nandi, Roy Homburg                                                                                                        | TOG                                                                                                                                                    |
| Review Internal podalic version with breech extraction                   | The article explores the historical and current use of internal podalic version with breech extraction, particularly for the delivery of a second twin, and discusses the associated risks, benefits, and training issues.                                          | 2011 | Sophia NE Webster, Andrew D Loughney                                                                                            | TOG                                                                                                                                                    |
| Developing a Green-top Guideline Guidance for developers                 | This document outlines the process for developing Green-top Guidelines by the Royal College of Obstetricians and Gynaecologists to support high-quality care in obstetrics and gynaecology.                                                                         | 2020 | Royal College of Obstetricians and Gynaecologists                                                                               | RCOG                                                                                                                                                   |

Continued on next page

Table 1 – continued from previous page

| Title                                                                                                                 | Synopsis                                                                                                                                                                                                                                    | Year | Authors                                                       | Publisher                                             |
|-----------------------------------------------------------------------------------------------------------------------|---------------------------------------------------------------------------------------------------------------------------------------------------------------------------------------------------------------------------------------------|------|---------------------------------------------------------------|-------------------------------------------------------|
| Urinary incontinence and pelvic organ prolapse in women: management                                                   | This guideline covers assessing and managing urinary incontinence and pelvic organ prolapse in women aged 18 and over, including complications associated with mesh surgery for these conditions.                                           | 2019 | –                                                             | NICE                                                  |
| Antenatal care                                                                                                        | This guideline covers the routine antenatal care that women and their babies should receive, aiming to ensure regular check-ups, information, and support for pregnant women.                                                               | 2021 | –                                                             | NICE                                                  |
| The Role of Natural Killer Cells in Human Fertility                                                                   | This paper reviews the function of natural killer cells in reproduction and provides recommendations for measuring these cells in women with reproductive failure.                                                                          | 2016 | Professor SM Laird, Dr GE Lash, Professor TC Li, et al.       | RCOG                                                  |
| Post-Hysterectomy Vaginal Vault Prolapse                                                                              | This guideline provides recommendations for the management of post-hysterectomy vaginal vault prolapse, including diagnosis, prevention, and treatment options.                                                                             | 2015 | –                                                             | RCOG/BSUG                                             |
| Vaginal mesh in prolapse surgery                                                                                      | The article reviews the use of vaginal mesh in pelvic organ prolapse surgery, discussing its history, types, risks, and current recommendations.                                                                                            | 2018 | Patrick Campbell, Swati Jha, Alfred Cutner                    | TOG                                                   |
| The key features of highly effective training units in obstetrics and gynaecology                                     | This article explores the characteristics of highly effective training units in obstetrics and gynaecology, focusing on reducing trainee attrition and improving educational environments.                                                  | 2020 | Marie O'Sullivan, Sarah Newell, Jonathan Frost, et al.        | TOG                                                   |
| WHO type 1 anovulation: an update on diagnosis, management and implications for long-term health                      | The article discusses WHO type 1 anovulatory disorders, their diagnosis, management, and implications for long-term health, focusing on conditions like hypogonadotrophic hypogonadism, hypothalamic amenorrhoea, and hypopituitarism.      | 2020 | Vikram Talaulikar, Ephraim Yasmin                             | TOG                                                   |
| Management of diabetic ketoacidosis in pregnancy                                                                      | This article discusses the challenges, diagnosis, management, and prevention of diabetic ketoacidosis in pregnancy, highlighting its serious implications for both mother and fetus.                                                        | 2017 | Manoj Mohan, Khaled Ahmed Mohamed Baagar, Stephen Lindow      | TOG                                                   |
| Differences of sexual development and their clinical implications                                                     | The article discusses the spectrum of conditions known as differences of sex development (DSD), their diagnosis, management, and the importance of multidisciplinary care.                                                                  | 2020 | Rhianna Davies, Lowri Davies, Djavaid Alleemudder, et al.     | TOG                                                   |
| Dealing with a serious incident requiring investigation in obstetrics and gynaecology: a training perspective         | This article reviews literature, guidance, and best practice recommendations for dealing with serious incidents requiring investigation (SIRIs) in obstetrics and gynaecology, focusing on training at trust, deanery, and national levels. | 2014 | Madeleine Macdonald, Radhika Gosakan, Alison E Cooper, et al. | TOG                                                   |
| Pregnancy following treatment for malignancy                                                                          | The article discusses the implications and management of pregnancy in women who have survived cancer and undergone treatments that may have long-term effects on various organs.                                                            | 2016 | Suzanne VF Wallace, Gill A Swallow                            | TOG                                                   |
| BCSH guideline for the use of anti-D immunoglobulin for the prevention of haemolytic disease of the fetus and newborn | This guideline provides practical guidance on the use of anti-D immunoglobulin to prevent Rh D alloimmunisation and haemolytic disease of the fetus and newborn.                                                                            | 2013 | H. Qureshi, E. Massey, D. Kirwan, et al.                      | British Committee for Standards in Haematology (BCSH) |
| The Management of Women with Red Cell Antibodies during Pregnancy                                                     | This guideline provides comprehensive management strategies for pregnant women with red cell antibodies, addressing fetal anaemia risks, monitoring, and transfusion requirements.                                                          | 2014 | –                                                             | RCOG                                                  |

Continued on next page

Table 1 – continued from previous page

| Title                                                                                            | Synopsis                                                                                                                                                                                                                                                                   | Year | Authors                                                        | Publisher   |
|--------------------------------------------------------------------------------------------------|----------------------------------------------------------------------------------------------------------------------------------------------------------------------------------------------------------------------------------------------------------------------------|------|----------------------------------------------------------------|-------------|
| Sex Steroid Treatment for Pubertal Induction and Replacement in the Adolescent Girl              | This paper discusses the use of sex steroid replacement for pubertal induction and replacement in adolescent girls with hypogonadism, focusing on timing, regimens, and considerations for treatment.                                                                      | 2013 | Dr G Conway MD FRCP, Professor HOD Critchley FRCOG             | RCOG        |
| Alternatives to HRT for the Management of Symptoms of the Menopause                              | This paper provides an updated review of alternatives to hormone replacement therapy (HRT) for managing menopausal symptoms, focusing on the efficacy and safety of various non-hormonal treatments.                                                                       | 2010 | Ms MCP Rees FRCOG and Mr N Panay MRCOG                         | RCOG        |
| The role of tubal patency tests and tubal surgery in the era of assisted reproductive techniques | This article reviews the current best available evidence and provides expert insight on the role of tubal patency tests and tubal surgery in the era of assisted reproductive techniques.                                                                                  | 2014 | Yalanadu N Suresh, Nitish N Narvekar                           | TOG         |
| Best practice in telemedicine for abortion care                                                  | This publication provides guidance on the provision of abortion care via telemedicine, emphasizing its safety, effectiveness, and the reduction of logistical barriers for patients.                                                                                       | 2022 | Sharon Cameron, Michelle Cooper, John Reynolds-Wright          | RCOG        |
| Pitfalls of prenatal diagnosis associated with mosaicism                                         | The article discusses the challenges and implications of non-invasive prenatal testing (NIPT) in detecting chromosomal mosaicism, particularly confined placental mosaicism, and the importance of accurate diagnosis and counselling.                                     | 2023 | Kelly Reilly, Samantha Doyle, Susan J Hamilton, et al.         | TOG         |
| The Management of Ovarian Cysts in Postmenopausal Women                                          | This guideline provides recommendations for the diagnosis, assessment, and management of ovarian cysts in postmenopausal women, emphasizing the differentiation between benign and malignant cysts to guide appropriate treatment strategies.                              | 2016 | –                                                              | RCOG        |
| Cystoscopy for the gynaecologist: how to do a cystoscopy                                         | This article provides a brief overview of the indications, contraindications, and procedural methods for performing cystoscopy in gynaecology.                                                                                                                             | 2017 | Margaret Lyttle, Gillian Fowler                                | TOG         |
| The management of vulval itching caused by benign vulval dermatoses                              | This article discusses patient assessment, vulval examination, and treatment of vulval diseases, focusing on dermatological conditions and emphasizing the importance of individualized management and referral to specialized services for complex cases.                 | 2017 | David Nunns, Rosalind Simpson, Andrew Watson, et al.           | TOG         |
| Abdominal incisions and sutures in obstetrics and gynaecology                                    | This article reviews various abdominal incisions, sutures, and closure methods used in obstetrics, benign gynaecology, and oncology practice, emphasizing the importance of individualized incision selection and the evaluation of traditional and new closure materials. | 2014 | Radhae Raghavan, Pallavi Arya, Prathibha Arya, et al.          | TOG         |
| Guidance 4. Colposcopic diagnosis, treatment and follow up                                       | This guidance provides updated standards and protocols for the diagnosis, treatment, and follow-up of cervical intraepithelial neoplasia (CIN) and early stage cervical cancer through colposcopy.                                                                         | 2024 | –                                                              | NHS England |
| Repair of Third- and Fourth-Degree Perineal Tears Following Childbirth                           | This paper provides advice for clinicians in obtaining consent for women undergoing repair of third- or fourth-degree perineal tears following childbirth.                                                                                                                 | 2010 | Dr KMK Ismail FRCOG and Professor C Kettle PhD Dip Mid SCM SRN | RCOG        |
| The management of urogynaecological problems in pregnancy and the postpartum period              | This article discusses the management of various urogynaecological issues such as stress urinary incontinence, overactive bladder, pelvic organ prolapse, recurrent urinary tract infections, and urinary retention during pregnancy and the postpartum period.            | 2022 | Faisal Karim, George Araklitis, Dudley Robinson, et al.        | TOG         |
| Diagnosis and management of premature ovarian failure                                            | The article discusses the causes, diagnosis, and management of premature ovarian failure, emphasizing the importance of multidisciplinary care and hormone replacement therapy.                                                                                            | 2011 | Puneet Arora, David W Polson                                   | TOG         |

Continued on next page

Table 1 – continued from previous page

| Title                                                                                  | Synopsis                                                                                                                                                                                                                                              | Year | Authors                                                                                   | Publisher        |
|----------------------------------------------------------------------------------------|-------------------------------------------------------------------------------------------------------------------------------------------------------------------------------------------------------------------------------------------------------|------|-------------------------------------------------------------------------------------------|------------------|
| OBTAINING VALID CONSENT FOR COMPLEX GYNAECOLOGICAL SURGERY                             | This guidance provides a framework for obtaining valid consent from women undergoing complex gynaecological surgery, emphasizing the importance of clear communication and understanding of risks and benefits.                                       | –    | Mr ADG Roberts<br>FRCOG                                                                   | RCOG             |
| Early ovarian ageing                                                                   | The article discusses early ovarian ageing (EOA), its prevalence, pathophysiology, effects on fertility, and potential management strategies, highlighting the importance of early identification and intervention.                                   | 2019 | Kate Maclaran,<br>Dimitrios Nikolaou                                                      | TOG              |
| A review of evidence-based management of uterine fibroids                              | This article reviews the clinical effectiveness of various treatments for symptomatic uterine fibroids in premenopausal women, focusing on reducing menstrual loss and fibroid size as well as improving symptoms.                                    | 2016 | Kinza Younas,<br>Essam Hadoura,<br>Franz Majoko, et al.                                   | TOG              |
| European Journal of Obstetrics & Gynecology and Reproductive Biology                   | This article provides expert opinions and guidelines on the management and prevention of ovarian cancer, focusing on risk assessment, surveillance, and surgical prevention strategies.                                                               | 2024 | Esther Moss,<br>Alexandra Taylor,<br>Adrian Andreou, et al.                               | Elsevier<br>B.V. |
| Pelvic congestion syndrome                                                             | Pelvic congestion syndrome is a poorly understood condition that contributes to chronic pelvic pain syndrome, affecting a significant number of women, yet remains underdiagnosed due to lack of awareness and diagnostic challenges.                 | 2013 | Mohamed Waseem<br>Osman, Ilias<br>Nikolopoulos,<br>Kannamannadiar<br>Jayaprakasan, et al. | TOG              |
| Early abdominal ectopic pregnancy: challenges, update and review of current management | The article discusses the challenges, updates, and current management strategies for early abdominal ectopic pregnancies, emphasizing the need for high suspicion for diagnosis and the complexities involved in medical and surgical management.     | 2014 | Nilesh Agarwal,<br>Funlayo Odejinmi                                                       | TOG              |
| Non-mesh surgery for stress urinary incontinence                                       | The article discusses the shift towards non-mesh surgical options for stress urinary incontinence (SUI) following concerns over mesh procedures, highlighting current practices, guidelines, and training requirements.                               | 2021 | Priyanka H Krishnaswamy,<br>Veenu Tyagi, Karen Lesley Guerrero                            | TOG              |
| Pregnancy and Breast Cancer                                                            | This guideline provides clinical guidance for managing pregnancy in women with a diagnosis or history of breast cancer, emphasizing a multidisciplinary approach.                                                                                     | 2011 | Ms MC Davies<br>FRCOG, Dr AL Jones                                                        | RCOG             |
| Natural killer cells and reproductive health                                           | The article explores the role of uterine natural killer cells in reproductive health, particularly their involvement in decidualisation, implantation, and potential links to reproductive disorders such as recurrent miscarriage and pre-eclampsia. | 2016 | Hsu Phern Chong,<br>Siobhan M Quenby                                                      | TOG              |
| Diagnosis and Management of Ectopic Pregnancy                                          | This guideline provides evidence-based recommendations for the diagnosis and management of various types of ectopic pregnancies, including tubal, cervical, caesarean scar, interstitial, cornual, ovarian, abdominal, and heterotopic pregnancies.   | 2016 | Elson CJ, Salim R,<br>Potdar N, et al.                                                    | RCOG             |
| Management of Breech Presentation                                                      | This guideline provides updated information on the management of breech presentation, focusing on decision-making regarding the mode of delivery and techniques used during delivery.                                                                 | 2017 | Impey LWM, Murphy DJ, Griffiths M, et al.                                                 | RCOG             |
| The diagnosis and management of fetal cardiac arrhythmias                              | This article reviews the diagnosis and management of fetal cardiac arrhythmias, highlighting the use of transplacental therapy and the importance of standardised protocols.                                                                          | 2022 | Daniel Stott, Pranav P Pandya, George Attilakos, et al.                                   | TOG              |
| Intrahepatic cholestasis of pregnancy                                                  | This guideline provides evidence-based recommendations for the diagnosis and management of intrahepatic cholestasis of pregnancy, focusing on maternal and fetal risks, and the importance of shared decision-making.                                 | 2022 | Joanna Girling,<br>Caroline L. Knight,<br>Lucy Chappell                                   | RCOG             |

Continued on next page

Table 1 – continued from previous page

| Title                                                                                                                                                       | Synopsis                                                                                                                                                                                                                                                   | Year | Authors                                                               | Publisher                                             |
|-------------------------------------------------------------------------------------------------------------------------------------------------------------|------------------------------------------------------------------------------------------------------------------------------------------------------------------------------------------------------------------------------------------------------------|------|-----------------------------------------------------------------------|-------------------------------------------------------|
| Stem Cell Therapies in Obstetrics and Gynaecology: The Female Urogenital Tract and the Fetus as Sources and Targets for Molecular and Regenerative Medicine | This paper reviews the progress and challenges of applying regenerative medicine to the urogenital tract and using stem cells for treating inherited genetic diseases with irreversible perinatal damage.                                                  | 2013 | Professor AJ Atala MD, Dr JKY Chan MRCOG, Dr M Choolani FRCOG, et al. | RCOG                                                  |
| Postpartum psychosis                                                                                                                                        | This article reviews postpartum psychosis, emphasizing the importance of recognizing high-risk women and the need for early recognition and prompt treatment of the illness.                                                                               | 2013 | Arianna Di Florio, Sue Smith, Ian Jones                               | TOG                                                   |
| Review Hormone replacement therapy and breast disease                                                                                                       | The article discusses the relationship between hormone replacement therapy (HRT) and breast cancer, highlighting the increased risk associated with the addition of progestogen, and examines the impact of HRT on mammography and breast cancer survival. | 2010 | Jo Marsden                                                            | TOG                                                   |
| Perinatal mental health services: Recommendations for the provision of services for childbearing women                                                      | This report outlines the provision of good-quality mental health services for women with moderate to severe mental illness during the perinatal period, emphasizing the need for specialist services and integrated care pathways.                         | 2021 | Sarah Taha, Cressida Manning, Hind Khalifeh, et al.                   | The Royal College of Psychiatrists                    |
| Morcellation for Myomectomy or Hysterectomy                                                                                                                 | This paper provides advice for healthcare professionals on obtaining consent from individuals undergoing myomectomy or hysterectomy for benign conditions, where the use of morcellation is being considered.                                              | 2019 | –                                                                     | RCOG                                                  |
| Child sexual exploitation: a guide for obstetricians and gynaecologists                                                                                     | This article provides guidance for obstetricians and gynaecologists on identifying and managing cases of child sexual exploitation (CSE), highlighting the importance of training, referral pathways, and joint working.                                   | 2017 | Katherine Gilmore, Laura Mitchell, Melinda Tenant-Flowers, et al.     | TOG                                                   |
| Endometriosis                                                                                                                                               | The guideline by the European Society of Human Reproduction and Embryology provides clinical recommendations for the diagnosis and treatment of endometriosis to improve healthcare delivery.                                                              | –    | –                                                                     | European Society of Human Reproduction and Embryology |
| Perimortem caesarean section – why, when and how                                                                                                            | This article explores the rationale, timing, and practical steps for performing perimortem caesarean sections to improve maternal survival during cardiac arrest in pregnancy.                                                                             | 2018 | Justin J Chu, Kim Hinshaw, Sara Paterson-Brown, et al.                | TOG                                                   |
